# Supplementary material for: Symmetry and Minimal Hamiltonian of Nonsymmorphic Collinear Antiferromagnet MnTe
Source: arXiv:2503.07951 source file (2025-03-11)
Supplement: Supplementary file 1 [file sm.pdf]

# Supplementary Materials: Symmetry and Minimal Hamiltonian of Nonsymmorphic Collinear Antiferromagnet MnTe

Koichiro Takahashi,[1,*] Hong-Fei Huang,[2,*] Jie-Xiang Yu,[2,†] and Jiadong Zang[1,‡]

[1]*Department of Physics and Astronomy, University of New Hampshire, Durham, New Hampshire 03824, USA*
[2]*School of Physical Science and Technology, Soochow University, Suzhou 215006, China*

## I. CRYSTAL STRUCTURE OF $\alpha$-MNTE

$\alpha$-type manganese telluride (MnTe) crystallizes in the NiAs-type (hexagonal) structure, which belongs to the space group $G = P_{6_3/mmc}$ (No. 194). This structure can be viewed as a hexagonal Bravais lattice with a four-sublattice basis (two Mn sites and two Te sites) in each unit cell. We define the following primitive lattice vectors:

$$\boldsymbol{a}_1 = \frac{1}{2}a\hat{\boldsymbol{x}} - \frac{\sqrt{3}}{2}a\hat{\boldsymbol{y}}, \quad \boldsymbol{a}_2 = \frac{1}{2}a\hat{\boldsymbol{x}} + \frac{\sqrt{3}}{2}a\hat{\boldsymbol{y}}, \quad \boldsymbol{a}_3 = c\hat{\boldsymbol{z}} \tag{S1}$$

where $a$ is the in-plane lattice constant and $c$ is the the out-of-plane lattice constant. The Bravais lattice is given by

$$\mathbf{R}(n_1, n_2, n_3) = n_1\boldsymbol{a}_1 + n_2\boldsymbol{a}_2 + n_3\boldsymbol{a}_3 \tag{S2}$$

where $n_1, n_2, n_3 \in \mathbb{Z}$. The sublattice basis of Te atoms labeled as $\boldsymbol{\tau}_A$ and $\boldsymbol{\tau}_B$ within a unit cell are given by

$$\boldsymbol{\tau}_A = \frac{a}{2}\hat{\boldsymbol{x}} + \frac{\sqrt{3}}{6}a\hat{\boldsymbol{y}} - \frac{c}{4}\hat{\boldsymbol{z}}, \quad \boldsymbol{\tau}_B = \frac{a}{2}\hat{\boldsymbol{x}} - \frac{\sqrt{3}}{6}a\hat{\boldsymbol{y}} + \frac{c}{4}\hat{\boldsymbol{z}}, \tag{S3}$$

The sublattice basis of Mn atoms labeled as $\boldsymbol{\tau}'_A$ and $\boldsymbol{\tau}'_B$ within a unit cell are given by

$$\boldsymbol{\tau}'_A = -\frac{c}{2}\hat{\boldsymbol{z}}, \quad \boldsymbol{\tau}'_B = \mathbf{0} \tag{S4}$$

where the alternate the magnetization along in-plane Néel vector. Then, the reciprocal primitive vectors are given by

$$\boldsymbol{b}_1 = \frac{2\pi}{\Omega}\boldsymbol{a}_2 \times \boldsymbol{a}_3 = \frac{2\pi}{\sqrt{3}a}\left(\sqrt{3}\hat{\boldsymbol{x}} - \hat{\boldsymbol{y}}\right), \quad \boldsymbol{b}_2 = \frac{2\pi}{\Omega}\boldsymbol{a}_3 \times \boldsymbol{a}_1 = \frac{2\pi}{\sqrt{3}a}\left(\sqrt{3}\hat{\boldsymbol{x}} + \hat{\boldsymbol{y}}\right), \quad \boldsymbol{b}_3 = \frac{2\pi}{\Omega}\boldsymbol{a}_1 \times \boldsymbol{a}_2 = \frac{2\pi}{c}\hat{\boldsymbol{z}} \tag{S5}$$

The whole first Brillouin zone $\mathbf{K}$ can be spanned by the primitive vectors.

$$\boldsymbol{K} = u\boldsymbol{b}_1 + v\boldsymbol{b}_2 + w\boldsymbol{b}_3 = k_x\hat{\boldsymbol{x}} + k_y\hat{\boldsymbol{y}} + k_z\hat{\boldsymbol{z}} \tag{S6}$$

and high-symmetry points in the first Brillouin zone are given below:

| Points | $(u, v, w)$ | $(k_x, k_y, k_z)$ |
|---|---|---|
| $\Gamma$ | $(0, 0, 0)$ | $(0, 0, 0)$ |
| $A$ | $(0, 0, \frac{1}{2})$ | $(0, 0, \frac{\pi}{c})$ |
| $K1$ | $(\frac{1}{3}, \frac{1}{3}, 0)$ | $(\frac{4\pi}{3a}, 0, 0)$ |
| $M1$ | $(0, \frac{1}{2}, 0)$ | $(\frac{\pi}{a}, \frac{\pi}{\sqrt{3}a}, 0)$ |
| $K2$ | $(\frac{1}{3}, 0, 0)$ | $(\frac{2\pi}{3a}, -\frac{2\pi}{\sqrt{3}a}, 0)$ |
| $M2$ | $(\frac{1}{2}, -\frac{1}{2}, 0)$ | $(0, -\frac{2\pi}{\sqrt{3}a}, 0)$ |
| $H1$ | $(\frac{1}{3}, \frac{1}{3}, \frac{\pi}{c})$ | $(\frac{4\pi}{3a}, 0, \frac{\pi}{c})$ |
| $L1$ | $(0, \frac{1}{2}, \frac{\pi}{c})$ | $(\frac{\pi}{a}, \frac{\pi}{\sqrt{3}a}, \frac{\pi}{c})$ |
| $H2$ | $(\frac{1}{3}, 0, \frac{\pi}{c})$ | $(\frac{2\pi}{3a}, -\frac{2\pi}{\sqrt{3}a}, \frac{\pi}{c})$ |
| $L2$ | $(\frac{1}{2}, -\frac{1}{2}, \frac{\pi}{c})$ | $(0, -\frac{2\pi}{\sqrt{3}a}, \frac{\pi}{c})$ |

* These authors contributed equally to this work.
† jxyu@suda.edu.cn
‡ jiadong.zang@unh.edu

where the length of the high-symmetric paths are given by

$$\overline{\Gamma A} = \frac{\pi}{c}, \quad \overline{\Gamma M1} = \frac{2\pi}{\sqrt{3}a}, \quad \overline{\Gamma K1} = \frac{4\pi}{3a}, \quad \overline{M1K1} = \frac{2\pi}{3a} \tag{S7}$$

## II. IRREDUCIBLE REPRESENTATION AND $k \cdot p$ HAMILTONIAN OF NON-SOC PARAMAGNETIC MNTE

Here, we review the way to construct the effective Hamiltonian of MnTe in non-magnetic case, at both Γ and $A$ point.

As discussed in the main text, for non-SOC paramagnetic MnTe, the relevant basis at the Γ point is formed by spinless $p_z$ orbitals on the $\boldsymbol{\tau}_A$ and $\boldsymbol{\tau}_B$ tellurium sublattices. In this representation, the symmetry generators at Γ act as follows:

$$D\left(\{3^-_{0001}|0\}\right) = \sigma_0, \quad D\left(\{2_{0001}|1/2\}\right) = \sigma_x, \quad D\left(\{2_{11\bar{2}0}|0\}\right) = -\sigma_x, \quad D\left(\mathcal{I}\right) = -\sigma_x \tag{S8}$$

where $\sigma$ denotes the Pauli matrices that encode the sublattice pseudospin $\{A, B\}$.

At the $A$ point, the relevant basis consists of spinless $p_x$ and $p_y$ orbitals on the $\boldsymbol{\tau}_A$ and $\boldsymbol{\tau}_B$ sublattices. The symmetry generators at $A$ act as:

$$D\left(\{3^-_{0001}|0\}\right) = \sigma_0\left(-\frac{1}{2}\tau_0 + \frac{\sqrt{3}}{2}i\tau_y\right), \quad D\left(\{2_{0001}|1/2\}\right) = i\sigma_y\tau_0, \quad D\left(\{2_{11\bar{2}0}|0\}\right) = \sigma_x\tau_z, \quad D\left(\mathcal{I}\right) = -\sigma_x \tag{S9}$$

where now $\sigma$ refers to the sublattice pseudospin and $\tau$ to the $\{p_x, p_y\}$ orbital pseudospin.

To enforce symmetry constraints, we require that for every group element $g \in G$,

$$D(g)h(g^{-1}\mathbf{k})D^{-1}(g) = h(\mathbf{k}) \tag{S10}$$

We can expand the effective Hamiltonian near a chosen high-symmetry point $\mathbf{k}$ (here, $\mathbf{k} = \Gamma$ or $A$) as

$$h(\mathbf{k}) = \sum_i \boldsymbol{P}_i(\mathbf{k}) \cdot \boldsymbol{B}_i \tag{S11}$$

where each $\boldsymbol{P}_i(\mathbf{k})$ is a polynomial vector in $\{k_x, k_y, k_z\}$, and $\{\boldsymbol{B}_i\}$ is a set of basis matrices formed by tensor products of Pauli matrices. Concretely,

$$\{\boldsymbol{B}_i\}^{\mathbf{k}=\Gamma} = \{\sigma_0, \sigma_x, \sigma_y, \sigma_z\}, \quad \{\boldsymbol{B}_i\}^{\mathbf{k}=A} = \{\sigma_0, \sigma_x, \sigma_y, \sigma_z\} \otimes \{\tau_0, \tau_x, \tau_y, \tau_z\} \tag{S12}$$

where ⊗ denotes the tensor product.

Substituting Eq. S11 into Eq. S10 for each $g \in G$, we have

$$D(g)\left(\sum_i \boldsymbol{P}_i(g^{-1}\mathbf{k}) \cdot \boldsymbol{B}_i\right)D^{-1}(g) = \sum_i \boldsymbol{P}_i(\mathbf{k}) \cdot \boldsymbol{B}_i \tag{S13}$$

This expression can be rearranged as

$$\sum_i \boldsymbol{P}_i(g^{-1}\mathbf{k}) \cdot D(g)\boldsymbol{B}_i D^{-1}(g) = \sum_i \boldsymbol{P}_i(\mathbf{k}) \cdot \boldsymbol{B}_i \tag{S14}$$

Thus, the only permissible terms in the effective Hamiltonian are those combinations of $\boldsymbol{P}_i(\mathbf{k})$ and $\boldsymbol{B}_i$ that satisfy, for all $g \in G$,

$$\eta(g)\boldsymbol{P}_i(\mathbf{k}) = \boldsymbol{P}_i(g^{-1}\mathbf{k}) \tag{S15}$$

$$\xi(g)\boldsymbol{B}_i = D(g)\boldsymbol{B}_i D^{-1}(g) \tag{S16}$$

$$\eta(g)\xi(g)^\dagger = E \tag{S17}$$

where $E$ is the identity matrix, $\eta(g)$ and $\xi(g)$ are the matrix factors arising from the symmetry operations, and their traces are directly related to those in Table S1. In this table, the leftmost columns list the irreducible representations of $D_{6h}$. Moving rightward, the table indicates the polynomials $\boldsymbol{P}(\mathbf{k})$ that transform under each irreducible representation (carrying the same matrix factor $\eta(g)$), then the basis functions $\boldsymbol{B}$ at the Γ point that share the corresponding factor $\xi(g)$, and finally the basis functions at the $A$ point that also carry $\xi(g)$. According to the symmetry constraints in the main text, only those $\boldsymbol{P}(\mathbf{k})$ and $\boldsymbol{B}$ appearing together in the same row can form permissible terms in the effective Hamiltonian.

| | $E$ | $\{3^-_{0001}\|0\}$ | $\{2_{0001}\|1/2\}$ | $\{2_{11\bar{2}0}\|0\}$ | $\mathcal{I}$ | | $\Gamma$ | $A$ |
|---|---|---|---|---|---|---|---|---|
| $A_{1g}$ | 1 | 1 | 1 | 1 | 1 | $x^2+y^2, z^2$ | $\sigma_0, \sigma_x$ | $\sigma_0\tau_0$ |
| $A_{1u}$ | 1 | 1 | 1 | 1 | -1 | | | $\sigma_y\tau_y$ |
| $A_{2g}$ | 1 | 1 | 1 | -1 | 1 | | | $\sigma_0\tau_y$ |
| $A_{2u}$ | 1 | 1 | 1 | -1 | -1 | $z$ | | $\sigma_y\tau_0$ |
| $B_{2g}$ | 1 | 1 | -1 | 1 | 1 | | | $\sigma_x\tau_0$ |
| $B_{2u}$ | 1 | 1 | -1 | 1 | -1 | | | $\sigma_z\tau_y$ |
| $B_{1g}$ | 1 | 1 | -1 | -1 | 1 | | | $\sigma_x\tau_y$ |
| $B_{1u}$ | 1 | 1 | -1 | -1 | -1 | | $\sigma_y, \sigma_z$ | $\sigma_z\tau_0$ |
| $E_{2g}$ | 2 | -1 | 2 | 0 | 2 | $(x^2-y^2, 2xy)$ | | $\sigma_0(\tau_z, \tau_x)$ |
| $E_{2u}$ | 2 | -1 | 2 | 0 | -2 | | | $\sigma_y(\tau_x, \tau_z), \sigma_z(\tau_x, \tau_z)$ |
| $E_{1g}$ | 2 | -1 | -2 | 0 | 2 | $(yz, xz)$ | | $\sigma_x(\tau_z, \tau_x)$ |
| $E_{1u}$ | 2 | -1 | -2 | 0 | -2 | $(x, y)$ | | |

Table S1. Irreducible representations of $D_{6h}$

Therefore, the full non-SOC paramagnetic effective Hamiltonians of MnTe around $\Gamma$ and $A$ points are given by

$$H^{\Gamma}_{\text{eff}} = c_1\left(k_x^2+k_y^2\right)+c_2k_z^2+c_3\left(k_x^2+k_y^2\right)\sigma_x+c_4k_z^2\sigma_x \tag{S18}$$

$$H^{A}_{\text{eff}} = c_1\left(k_x^2+k_y^2\right)+c_2k_z^2+c_3k_z\sigma_y+c_4\left[\left(k_x^2-k_y^2\right)\tau_z+2k_xk_y\tau_x\right]+c_5\left(k_xk_z\sigma_x\tau_x+k_yk_z\sigma_x\sigma_x\right) \tag{S19}$$

where we omit identity matrices $\sigma_0$ and $\tau_0$. The coefficients $c_1, c_2, c_3, c_4$, and $c_5$ are independent, and there is no requirement that they coincide for the $\Gamma$ and $A$ points.

The methods outlined here for the non-magnetic case provide a straightforward illustration of our approach. In the main text, we extend these techniques to treat the more complex AFM phases, both with and without SOC, where the Néel vector lies along various in-plane directions—the principal focus of this work. Note also that when anti-unitary time-reversal symmetry enters the group, the invariance condition is modified, as described in Section. II(B) of the main text.

## III. TIGHT-BINDING MODELING OF VALENCE TOP BANDS OF MNTE IN $p$-ORBITAL BASIS

Here, we construct the effective Hamiltonian in the sub-Hilbert space near the Fermi surface, which governs the electron transport properties in hole-doped MnTe. Since MnTe is a semiconductor, the tight-binding Linear Combination of Atomic Orbitals (LCAO) method is a suitable description. The sub-Hilbert space near the Fermi surface is effectively spanned by the Bloch states of $(5p)$-orbitals of $Te^{2-}$ with two basis $A$ and $B$ in a unit cell, i.e.

$$\{|p^A_{x\uparrow}\rangle, |p^A_{y\uparrow}\rangle, |p^A_{z\uparrow}\rangle, |p^B_{x\uparrow}\rangle, |p^B_{y\uparrow}\rangle, |p^B_{z\uparrow}\rangle, |p^A_{x\downarrow}\rangle, |p^A_{y\downarrow}\rangle, |p^A_{z\downarrow}\rangle, |p^B_{x\downarrow}\rangle, |p^B_{y\downarrow}\rangle, |p^B_{z\downarrow}\rangle\} \tag{S20}$$

To construct a minimum Hamiltonian, whose eigenvalues are the energy bands right below the Fermi surface, our general model is

$$H = H_{\text{Te-Te}} + H_{\text{Te-Mn}} + H_{\text{Mn-Mn}} + H_{\text{SOC}} \tag{S21}$$

where

$$\begin{aligned} H_{\text{Te-Te}} =& \sum_{\sigma}\sum_{i,\tau}\sum_{n}\epsilon_{pn}\, p^{\dagger}_{ni\tau\sigma}p_{ni\tau\sigma} + \sum_{\sigma}\sum_{n,n'}\sum_{<i,j>}\sum_{\tau\neq\tau'}{}' t_1\, p^{\dagger}_{ni\tau\sigma}p_{n'j\tau'\sigma} \\ &+ \sum_{\sigma}\sum_{n,n'}\sum_{\ll i,j\gg}\sum_{\tau} t_2\, p^{\dagger}_{ni\tau\sigma}p_{n'j\tau\sigma} + \sum_{\sigma}\sum_{n,n'}\sum_{\lll i,j\ggg}\sum_{\tau\neq\tau'}{}' t_3^{\sigma}\, p^{\dagger}_{ni\tau\sigma}p_{n'j\tau'\sigma} + H.c. \end{aligned} \tag{S22}$$

$$H_{\text{Te-Mn}} = \sum_{\sigma}\sum_{n,n'}\sum_{<i,j>}\sum_{\tau\neq\tau'}{}' t^{\sigma}_{pd}\, p^{\dagger}_{ni\tau\sigma}d_{n'j\tau'\sigma} + H.c. \tag{S23}$$

$$H_{\text{SOC}} = \lambda_{\text{SOC}}\sum_{i,\tau}\sum_{\sigma,\sigma'}\sum_{n,n'}\langle n\sigma|\mathbf{l}\cdot\mathbf{s}\,|n'\sigma'\rangle\; p^{\dagger}_{ni\tau\sigma}p_{n'i\tau\sigma'} + H.c. \tag{S24}$$

$$H_{\text{Mn-Mn}} = \sum_{\sigma}\sum_{i,\tau}\sum_{n}\epsilon_{dn}\, d^{\dagger}_{ni\tau\sigma}d_{ni\tau\sigma} \tag{S25}$$

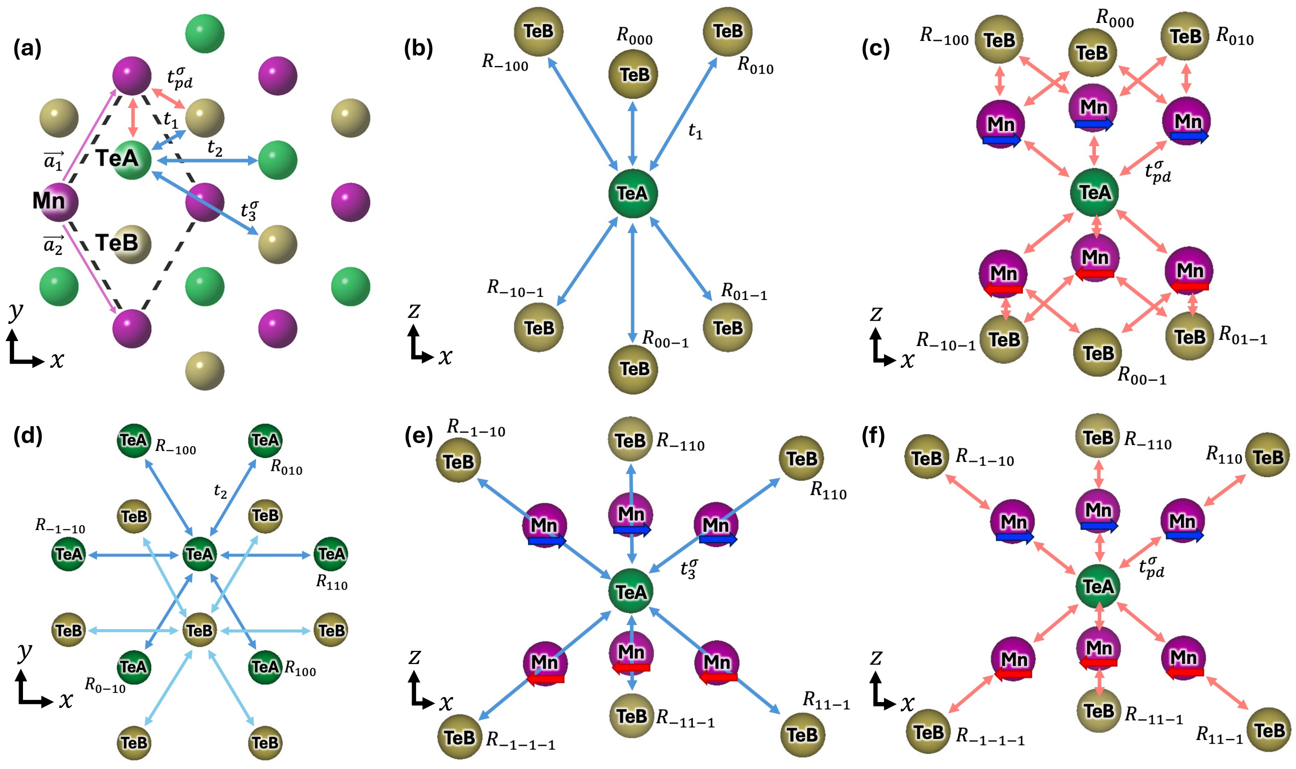


Figure S1. (a) Schematic diagram illustrating the Te–Te hopping pathways and the role of $t_{pd}$. The direct Te–Te hoppings include first-nearest ($t_1$), second-nearest ($t_2$), and third-nearest ($t_3$) processes, all of which are mediated by the Te–Mn hopping $t_{pd}$. Panels (b)–(f) depict individual hopping processes: (b) direct first-nearest Te–Te hopping ($t_1$); (c) manganese-mediated first-nearest Te–Te hopping via $t_{pd}$; (d) direct second-nearest Te–Te hopping ($t_2$); (e) direct third-nearest Te–Te hopping ($t_3$); and (f) manganese-mediated third-nearest Te–Te hopping via $t_{pd}$. Although Mn also mediates the second-nearest neighbor hoppings, their schematic representation is omitted. In panels (b)–(f), the label $R_{n_1n_2n_3}$ indicates the shift in unit-cell indices between the original site and the destination site.

Here, $p^{(\dagger)}_{ni\tau\sigma}$ and $d^{(\dagger)}_{ni\tau\sigma}$ denote the creation (annihilation) operators for electrons in the $p_n$ and $d_n$ orbitals, respectively, in the $i$-th unit cell at sublattice $\tau$ with spin $\sigma$. The index $n$ labels the orbital type: $x$, $y$, or $z$ for $p$-orbitals, and $xy, yz, zx, x^2-y^2$, or $z^2$ for $d$-orbitals. To simplify our model, we only include $z^2$ for $d$-orbitals. The parameters $\epsilon_{pn}$ and $\epsilon_{dn}$ represent the on-site energies for the $p$- and $d$-orbitals, respectively. The symbol $\tau$ distinguishes the two sublattice sites $\{A, B\}$ within the unit cell, and $\sigma$ denotes the electron spin ($\uparrow$, $\downarrow$). In the expressions above, $t_1$, $t_2$, and $t_3^\sigma$ denote the direct Te-Te hopping amplitudes between first, second, and third nearest neighbors, respectively (with the notation $< i, j >$ for first nearest neighbors, $\ll i, j \gg$ for second nearest neighbors, and $\lll i, j \ggg$ for third nearest neighbors). Notably, the hopping amplitude $t_3^\sigma$ is spin-dependent because the corresponding hopping channel involves a Mn atom with alternating magnetization layer by layer. Similarly, $t_{pd}^\sigma$ represents the hopping amplitude between Te $p$-orbitals and Mn $d$-orbitals, and is naturally spin-dependent. Here, the notation $< i, j >$ also applies to first-nearest neighbor Te-Mn hoppings.

The annihilation operators of Bloch states are given by the Fourier transformation of the annihilation operators of corresponding atomic orbitals at all unit cells,

$$p_{\mathbf{k}n\tau\sigma} = \frac{1}{\sqrt{N}} \sum_j e^{i\mathbf{k}\cdot\mathbf{R}_j} p_{nj\tau\sigma} \tag{S26}$$

$$d_{\mathbf{k}n\tau\sigma} = \frac{1}{\sqrt{N}} \sum_j e^{i\mathbf{k}\cdot\mathbf{R}_j} d_{nj\tau\sigma} \tag{S27}$$

Substituting the transformation above, our Hamiltonian reduces to

$$H = \sum_{\mathbf{k}} H^{\mathbf{k}}, \quad H^{\mathbf{k}} = H^{\mathbf{k}}_{\text{Te-Te}} + H^{\mathbf{k}}_{\text{Te-Mn}} + H^{\mathbf{k}}_{\text{Mn-Mn}} + H_{\text{SOC}} \tag{S28}$$

where

$$
\begin{aligned}
H^{\mathbf{k}}_{\text{Te-Te}} =& \sum_{\sigma}\sum_{\tau}\sum_{n} \epsilon_{pn}\, p^{\dagger}_{\mathbf{k}n\tau\sigma} p_{\mathbf{k}n\tau\sigma} + \sum_{\sigma}\sum_{n,n'}\sum_{\Delta\mathbf{R}_1}\sum_{\tau\neq\tau'}{}' t_1(\Delta\mathbf{R}_1)\, e^{i\mathbf{k}\cdot\Delta\mathbf{R}_1}\, p^{\dagger}_{\mathbf{k}n\tau\sigma} p_{\mathbf{k}n'\tau'\sigma} \\
&+ \sum_{\sigma}\sum_{n,n'}\sum_{\Delta\mathbf{R}_2}\sum_{\tau} t_2(\Delta\mathbf{R}_2)\, e^{i\mathbf{k}\cdot\Delta\mathbf{R}_2}\, p^{\dagger}_{\mathbf{k}n\tau\sigma} p_{\mathbf{k}n'\tau\sigma} + \sum_{\sigma}\sum_{n,n'}\sum_{\Delta\mathbf{R}_3}\sum_{\tau\neq\tau'}{}' t^{\sigma}_3(\Delta\mathbf{R}_3)\, e^{i\mathbf{k}\cdot\Delta\mathbf{R}_3}\, p^{\dagger}_{\mathbf{k}n\tau\sigma} p_{\mathbf{k}n'\tau'\sigma} + H.c. \quad \text{(S29)}\\
H^{\mathbf{k}}_{\text{Te-Mn}} =& \sum_{\sigma}\sum_{n,n'}\sum_{\Delta\mathbf{R}'_1}\sum_{\tau\neq\tau'}{}' t^{\sigma}_{pd}(\Delta\mathbf{R}'_1)\, e^{i\mathbf{k}\cdot\Delta\mathbf{R}_1}\, p^{\dagger}_{\mathbf{k}n\tau\sigma} d_{\mathbf{k}n'\tau'\sigma} + H.c. \quad \text{(S30)}\\
H_{\text{SOC}} =& \lambda_{\text{SOC}} \sum_{\tau}\sum_{\sigma,\sigma'}\sum_{n,n'} \langle n\sigma|\, \boldsymbol{l}\cdot\boldsymbol{s}\, |n'\sigma'\rangle\, p^{\dagger}_{\mathbf{k}n\tau\sigma} p_{\mathbf{k}n'\tau\sigma'} + H.c. \quad \text{(S31)}\\
H^{\mathbf{k}}_{\text{Mn-Mn}} =& \sum_{\sigma}\sum_{\tau}\sum_{n} \epsilon_{dn}\, d^{\dagger}_{\mathbf{k}n\tau\sigma} d_{\mathbf{k}n\tau\sigma} \quad \text{(S32)}
\end{aligned}
$$

Note that the summations over $\Delta\mathbf{R}_1$, $\Delta\mathbf{R}_2$, $\Delta\mathbf{R}_3$, and $\Delta\mathbf{R}'_1$ run over all the shift vectors corresponding to the nearest-neighbor translation of the unit cell during the hopping process. In the next chapter, we will derive these hopping parameters in detail using the Slater–Koster parametrization. By treating $H^{\mathbf{k}}_{\text{Te-Mn}}$ as a perturbation and performing the Schrieffer-Wolff transformation, one can get an effective Hamiltonian involving tellurium (5p) orbitals only. One can write the resulting Hamiltonian as

$$
H^{\mathbf{k}}_{h} = H^{\mathbf{k}}_{\text{Te-Te}} + \Delta H^{\mathbf{k}(2)}_{\text{Te-Mn}} \quad \text{(S33)}
$$

where $\Delta H^{\mathbf{k}(2)}_{\text{Te-Mn}}$ is the correction from Mn-mediated pseudo-hopping. In general,

$$
\Delta H^{\mathbf{k}(2)}_{\text{Te-Mn}} = \frac{H^{\mathbf{k}}_{\text{Te-Mn}} H^{\mathbf{k}\dagger}_{\text{Te-Mn}}}{\epsilon_p - H^{\mathbf{k}}_{\text{Mn-Mn}}} \quad \text{(S34)}
$$

Since direct hopping between Mn is neglected, $H^{\mathbf{k}}_{\text{Mn-Mn}}$ is diagonal and the Schrieffer-Wolff transformation is reduced to

$$
\Delta H^{\mathbf{k}(2)}_{\text{Te-Mn}} = \frac{H^{\mathbf{k}}_{\text{Te-Mn}} H^{\mathbf{k}\dagger}_{\text{Te-Mn}}}{\epsilon_p - \epsilon_d} \quad \text{(S35)}
$$

The formula above is equivalent to treating the second-order correction as the paired products of $pd$-hopping parameters, which describe the electron's hopping from a initial Te site to a final Te site mediated by a Mn site. As a result, the structure factor of these hoppings are the same as the corresponding direct Te-Te hoppings. From the above, the total $p$-orbital tight-binding Hamiltonian is given by

$$
\begin{aligned}
H^{\mathbf{k}}_{p} &= H^{\mathbf{k}}_{h} + H_{\text{SOC}} \quad \text{(S36)}\\
&= H^{\mathbf{k}}_{\text{Te-Te}} + \frac{H^{\mathbf{k}}_{\text{Te-Mn}} H^{\mathbf{k}\dagger}_{\text{Te-Mn}}}{\epsilon_p - \epsilon_d} + H_{\text{SOC}} \quad \text{(S37)}
\end{aligned}
$$

## IV. SLATER-KOSTER PARAMETRIZATION OF HOPPING MATRIX ELEMENTS

The hopping parameters are determined by Slater-Koster symmetry principle [1, 2] in terms of the directional cosines $(l, m, n)$ of the relative position vector $\mathbf{n}$, which is defined as

$$
\boldsymbol{n} = \left(\mathbf{r}_i - \mathbf{r}_f\right)/|\mathbf{r}_i - \mathbf{r}_f| = l\,\hat{\boldsymbol{x}} + m\,\hat{\boldsymbol{y}} + n\,\hat{\boldsymbol{z}} \quad \text{(S38)}
$$

where $\mathbf{r}_i$ and $\mathbf{r}_f$ is the position vector of the initial and final sites through the electron hopping. The hopping integral $t_{o_i,o_f}(l, m, n)$ where $o_i$ and $o_f$ are the orbital at $\mathbf{r}_i$ and the orbital at $\mathbf{r}_f$, respectively, can be obtained from the formulae in Ref. [1], in terms of two disposable parameters describing $\pi$-bonding $V_\pi$ and $\sigma$-bonding $V_\sigma$. Here, we denote the orbitals $p_x \to x, p_y \to y, p_z \to z,$

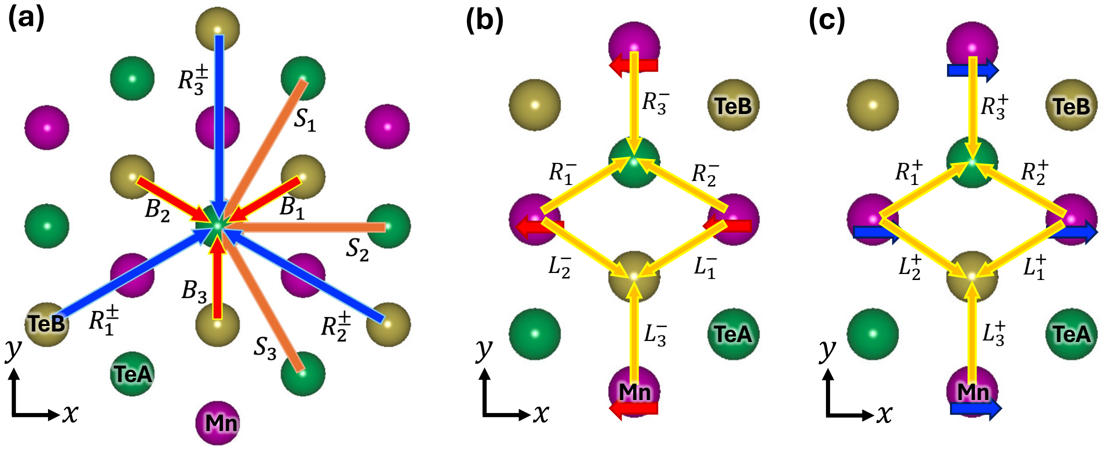


Figure S2. (a) shows the directional cosines for direct Te-Te hoppings. (b) shows the directional cosines for first-nearest neighbor Te-Mn hoppings via the lower layer of the original $A$ sublattice, and (c) shows the directional cosines for first-nearest neighbor Te-Mn hoppings via the upper layer of the original $A$ sublattice.

and $d_{z^2} \rightarrow z^2$.

$$t_{x,x}(\boldsymbol{n}) = l^2 V_{pp\sigma} + \left(1 - l^2\right) V_{pp\pi} \tag{S39}$$

$$t_{x,y}(\boldsymbol{n}) = lm\left(V_{pp\sigma} - V_{pp\pi}\right) \tag{S40}$$

$$t_{x,z^2}(\boldsymbol{n}) = l\left(n^2 - \frac{1}{2}\left(l^2 + m^2\right)\right) V_{pd\sigma} - \sqrt{3} l n^2 V_{pd\pi} \tag{S41}$$

$$t_{y,z^2}(\boldsymbol{n}) = m\left(n^2 - \frac{1}{2}\left(l^2 + m^2\right)\right) V_{pd\sigma} - \sqrt{3} m n^2 V_{pd\pi} \tag{S42}$$

$$t_{z,z^2}(\boldsymbol{n}) = n\left(n^2 - \frac{1}{2}\left(l^2 + m^2\right)\right) V_{pd\sigma} + \sqrt{3} n\left(l^2 + m^2\right) V_{pd\pi} \tag{S43}$$

Figure. S2 illustrates the directional cosines associated with the relative position vectors between neighboring Te atoms and between Te and Mn atoms.

To express the directional cosines for the relevant Te–Te and Te–Mn bonds, we first define the angles $\gamma$ and $\alpha$ based on the lattice constants $a$ and $c$. Specifically, $\gamma$ governs the first- and second-nearest neighbor Te–Te bonds via

$$\xi = \sqrt{\left(\frac{a}{\sqrt{3}}\right)^2 + \left(\frac{c}{2}\right)^2}, \quad \gamma = \cos^{-1}\left(\frac{a}{\sqrt{3}\xi}\right) \tag{S44}$$

while $\alpha$ describes the third-nearest neighbor Te–Te bonds and the first-nearest neighbor Te–Mn bonds through

$$\eta = \sqrt{\left(\frac{a}{\sqrt{3}}\right)^2 + \left(\frac{c}{4}\right)^2}, \quad \alpha = \cos^{-1}\left(\frac{a}{\sqrt{3}\eta}\right) \tag{S45}$$

In particular, the directional cosines for the first-nearest neighbor Te–Te pairs are given by

$$B_1 = \left(\frac{\sqrt{3}}{2}\cos\gamma, \frac{1}{2}\cos\gamma, -\sin\gamma\right), \quad B_2 = \left(\frac{\sqrt{3}}{2}\cos\gamma, -\frac{1}{2}\cos\gamma, -\sin\gamma\right), \quad B_3 = (0, \cos\gamma, -\sin\gamma) \tag{S46}$$

For the second-nearest neighbor Te–Te pairs, the directional cosines are

$$S_1 = \left(\frac{1}{2}, \frac{\sqrt{3}}{2}, 0\right), \quad S_2 = (1, 0, 0), \quad S_3 = \left(\frac{1}{2}, -\frac{\sqrt{3}}{2}, 0\right) \tag{S47}$$

For the third-nearest neighbor Te–Te pairs, as well as for the first-nearest neighbor Te–Mn pairs, the directional cosines are parameterized by the angle $\alpha$. They are given by

$$R_1^{\pm} = \left(\frac{\sqrt{3}}{2}\cos\alpha, \frac{1}{2}\cos\alpha, \mp\sin\alpha\right), \quad R_2^{\pm} = \left(-\frac{\sqrt{3}}{2}\cos\alpha, \frac{1}{2}\cos\alpha, \mp\sin\alpha\right), \quad R_3^{\pm} = (0, -\cos\alpha, \mp\sin\alpha) \tag{S48}$$

$$L_1^{\pm} = \left(-\frac{\sqrt{3}}{2}\cos\alpha, -\frac{1}{2}\cos\alpha, \pm\sin\alpha\right), \quad L_2^{\pm} = \left(\frac{\sqrt{3}}{2}\cos\alpha, -\frac{1}{2}\cos\alpha, \pm\sin\alpha\right), \quad L_3^{\pm} = (0, \cos\alpha, \pm\sin\alpha) \tag{S49}$$

In these expressions, the superscripts + and − distinguish between hoppings through the upper layer and lower layer of the original sublattice at A, respectively.

Given all the directional cosines of neighboring sites above, one can calculate the hopping matrix elements by using the Slater-Koster $\sigma$-bonding and $\pi$-bonding parameters, given by

$$\{V_{1pp\sigma}, V_{1pp\pi}, V_{2pp\sigma}, V_{2pp\pi}, V^{\pm}_{3pp\sigma}, V^{\pm}_{3pp\pi}, V^{\pm}_{pd\sigma}, V^{\pm}_{pd\pi}\} \tag{S50}$$

where we extended the SK parameters for the third nearest hopping between Te and Te, and the first nearest hopping between Te and Mn as different values for the electrons' spin, taking into account the minimum correction of the effects from antiferromagnetic Mn layers.

Here, we introduce the original SK parameters and lattice constants

$$\{a, c, \epsilon_p, \epsilon_p - \epsilon_d, V^{\pm}_{pd\sigma}, V^{\pm}_{pd\pi}, V_{1pp\sigma}, V_{1pp\pi}, V_{2pp\sigma}, V_{2pp\pi}, V^{\pm}_{3pp\sigma}, V^{\pm}_{3pp\pi}\} \tag{S51}$$

We convert the parameters into suitable forms to fit with the matrix values obtained by the DFT calculation.

$$c_3 = \cos^2\gamma, \quad c_4 = \cos^2\alpha, \quad \rho = \sqrt{c_3(1-c_3)} = \sin\gamma\cos\gamma, \quad \chi = \sqrt{c_4(1-c_4)} = \sin\alpha\cos\alpha \tag{S52}$$

$$V'^{\pm}_{pd\sigma} = \left(-\frac{1}{2}\cos^2\alpha + \sin^2\alpha\right)V^{\pm}_{pd\sigma}, \quad V'^{\pm}_{pd\pi} = \sqrt{3}\cos\alpha\sin\alpha\, V^{\pm}_{pd\pi}, \quad V'^{\pm}_{pd\sigma} = r_{\pm}\cos\beta_{\pm}, \quad V'^{\pm}_{pd\pi} = r_{\pm}\sin\beta_{\pm} \tag{S53}$$

$$\delta_{\pm} = \alpha + \beta_{\pm}, \quad \lambda_{\pm} = \frac{r^2_{\pm}}{\epsilon_p - \epsilon_d} < 0, \quad c_1^{\pm} = \lambda_{\pm}\sin^2\delta_{\pm} < 0, \quad c_2^{\pm} = \frac{1}{\tan\delta_{\pm}} \tag{S54}$$

$$g_1 = c_1^+ + c_1^-, \quad \tilde{g}_2^+ = -\tilde{g}_2^- = c_1^+c_2^+ - c_1^-c_2^-, \quad g_2^{\pm} = \frac{\tilde{g}_2^{\pm}}{g_1}, \quad \lambda_g = \lambda_+ + \lambda_- \tag{S55}$$

As a result, we write down the hopping matrices using the parameters below:

$$\{a, c, \epsilon_p, \lambda_{\pm}, c_1^{\pm}, c_2^{\pm}, V_{1pp\sigma}, V_{1pp\pi}, V_{2pp\sigma}, V_{2pp\pi}, V^{\pm}_{3pp\sigma}, V^{\pm}_{3pp\pi}\} \tag{S56}$$

where $g_1$, $g_2$ and $\lambda_g$ are used for intra-layer indirect hoppings, whose mediated antiferromagnetic channels are both up and down Mn layers. Note that $g_1$ and $\lambda_g$ is symmetric but $g_2^{\pm}$ is anti-symmetric under flipping the spin. The third-nearest direct hopping $V^{\pm}_{3pp\sigma}, V^{\pm}_{3pp\pi}$ will be strongly affected by the antiferromagnetic channels since a Mn site is in a straight line with two Te sites, thus we use the different parameters for the different spins.

Once we have all the hopping matrices, we can construct the full hopping Hamiltonian by multiplying each matrix with the corresponding phase factor $e^{i\mathbf{k}\cdot\Delta\mathbf{R}}$ associated with the shift vector of the Bravais lattice and summing over all terms, including their Hermitian conjugates. Here, we define the shift vector $\Delta\mathbf{R}$ specifying the position of a unit cell as

$$\Delta\mathbf{R}(n_1, n_2, n_3) = \mathbf{R}_f - \mathbf{R}_i = n_1\boldsymbol{a}_1 + n_2\boldsymbol{a}_2 + n_3\boldsymbol{a}_3 \tag{S57}$$

where $\mathbf{R}_i$ and $\mathbf{R}_f$ are the part of the Bravais lattice vector in the initial and final site position vectors, respectively.

$$\mathbf{r}_i = \mathbf{R}_i + \boldsymbol{\tau}_{A,B}, \quad \mathbf{r}_f = \mathbf{R}_f + \boldsymbol{\tau}_{A,B} \tag{S58}$$

We define the notation of a block $6\times 6$ hopping matrix of the Te basis $X, Y \in \{A, B\}$, as follows:

$$t^{XY}_{\Delta\mathbf{R}(n_1,n_2,n_3)} = \begin{pmatrix} t^{XY\uparrow}_{\Delta\mathbf{R}(n_1,n_2,n_3)} & \mathbf{0}_{3\times3} \\ \mathbf{0}_{3\times3} & t^{XY\downarrow}_{\Delta\mathbf{R}(n_1,n_2,n_3)} \end{pmatrix} \tag{S59}$$

Here, $t^{XY\uparrow}_{\Delta\mathbf{R}(n_1,n_2,n_3)}$ and $t^{XY\downarrow}_{\Delta\mathbf{R}(n_1,n_2,n_3)}$ represent the hopping matrices for spin-up and spin-down electrons, respectively, associated with the translation $\Delta\mathbf{R}(n_1, n_2, n_3)$ between unit cells. The off-diagonal zero matrices indicate that there is no hopping process which flips the electron's spin in the absence of spin–orbit coupling (SOC).

Then, the hopping Hamiltonian can be written as a $12\times 12$ matrix

$$H^{\mathbf{k}}_{h} = H^{\mathbf{k}}_{\text{Te−Te}} + \Delta H^{\mathbf{k}(2)}_{\text{Te−Mn}} = \sum_{n_1,n_2,n_3} e^{i\mathbf{k}\cdot\Delta\mathbf{R}(n_1,n_2,n_3)} \begin{pmatrix} t^{AA}_{\Delta\mathbf{R}(n_1,n_2,n_3)} & t^{BA}_{\Delta\mathbf{R}(n_1,n_2,n_3)} \\ t^{AB}_{\Delta\mathbf{R}(n_1,n_2,n_3)} & t^{BB}_{\Delta\mathbf{R}(n_1,n_2,n_3)} \end{pmatrix} \tag{S60}$$

$$= H^{\mathbf{k}}_{h_1} + H^{\mathbf{k}}_{h_2} + H^{\mathbf{k}}_{h_3} + H.c. \tag{S61}$$

where

$$H^{\mathbf{k}}_{h_1} = \begin{pmatrix} 0 & e^{i\mathbf{k}\cdot\Delta\mathbf{R}(0,0,1)}\, t^{BA}_{\Delta\mathbf{R}(0,0,1)} + e^{i\mathbf{k}\cdot\Delta\mathbf{R}(0,-1,1)}\, t^{BA}_{\Delta\mathbf{R}(0,-1,1)} + e^{i\mathbf{k}\cdot\Delta\mathbf{R}(1,0,1)}\, t^{BA}_{\Delta\mathbf{R}(1,0,1)} \\ e^{i\mathbf{k}\cdot\Delta\mathbf{R}(0,0,0)}\, t^{AB}_{\Delta\mathbf{R}(0,0,0)} + e^{i\mathbf{k}\cdot\Delta\mathbf{R}(0,1,0)}\, t^{AB}_{\Delta\mathbf{R}(0,1,0)} + e^{i\mathbf{k}\cdot\Delta\mathbf{R}(-1,0,0)}\, t^{AB}_{\Delta\mathbf{R}(-1,0,0)} & 0 \end{pmatrix} \tag{S62}$$

$$H^{\mathbf{k}}_{h_2} = \begin{pmatrix} e^{i\mathbf{k}\cdot\Delta\mathbf{R}(1,0,0)}\, t^{AA}_{\Delta\mathbf{R}(1,0,0)} + e^{i\mathbf{k}\cdot\Delta\mathbf{R}(1,1,0)}\, t^{AA}_{\Delta\mathbf{R}(1,1,0)} + e^{i\mathbf{k}\cdot\Delta\mathbf{R}(0,1,0)}\, t^{AA}_{\Delta\mathbf{R}(0,1,0)} & 0 \\ 0 & e^{i\mathbf{k}\cdot\Delta\mathbf{R}(1,0,0)}\, t^{BB}_{\Delta\mathbf{R}(1,0,0)} + e^{i\mathbf{k}\cdot\Delta\mathbf{R}(1,1,0)}\, t^{BB}_{\Delta\mathbf{R}(1,1,0)} + e^{i\mathbf{k}\cdot\Delta\mathbf{R}(0,1,0)}\, t^{BB}_{\Delta\mathbf{R}(0,1,0)} \end{pmatrix} \tag{S63}$$

$$H^{\mathbf{k}}_{h_3} = \begin{pmatrix} 0 & e^{i\mathbf{k}\cdot\Delta\mathbf{R}(-1,-1,1)}\, t^{BA}_{\Delta\mathbf{R}(-1,-1,1)} + e^{i\mathbf{k}\cdot\Delta\mathbf{R}(1,-1,1)}\, t^{BA}_{\Delta\mathbf{R}(1,-1,1)} + e^{i\mathbf{k}\cdot\Delta\mathbf{R}(1,1,1)}\, t^{BA}_{\Delta\mathbf{R}(1,1,1)} \\ e^{i\mathbf{k}\cdot\Delta\mathbf{R}(1,1,0)} t^{AB}_{\Delta\mathbf{R}(1,1,0)} + e^{i\mathbf{k}\cdot\Delta\mathbf{R}(-1,1,0)}\, t^{AB}_{\Delta\Delta\mathbf{R}(-1,1,0)} + e^{i\mathbf{k}\cdot\Delta\mathbf{R}(-1,-1,0)}\, t^{AB}_{\Delta\mathbf{R}(-1,-1,0)} & 0 \end{pmatrix} \tag{S64}$$

The on-site spin-orbit coupling matrix of $p$-orbitals $H_{\text{SOC}}$ with each basis of spin are given as below, note that the order of the basis are

$$\{|p^A_{z\uparrow}\rangle, |p^A_{x\uparrow}\rangle, |p^A_{y\uparrow}\rangle, |p^A_{z\downarrow}\rangle, |p^A_{x\downarrow}\rangle, |p^A_{y\downarrow}\rangle, |p^B_{z\uparrow}\rangle, |p^B_{x\uparrow}\rangle, |p^B_{y\uparrow}\rangle, |p^B_{z\downarrow}\rangle, |p^B_{x\downarrow}\rangle, |p^B_{y\downarrow}\rangle\} \tag{S65}$$

where spin quantization axis is along the Néel vector along $[11\bar{2}0]$ $(x)$ direction or $[1\bar{1}00]$ $(y)$ direction.

$$H^{[11\bar{2}0]}_{\text{SOC}} = \sigma_0 \otimes \frac{\lambda_{\text{SOC}}}{2} \begin{pmatrix} 0 & 0 & i & 0 & 1 & 0 \\ 0 & 0 & 0 & -1 & 0 & -i \\ -i & 0 & 0 & 0 & i & 0 \\ 0 & -1 & 0 & 0 & 0 & -i \\ 1 & 0 & -i & 0 & 0 & 0 \\ 0 & i & 0 & i & 0 & 0 \end{pmatrix}; \quad H^{[1\bar{1}00]}_{\text{SOC}} = \sigma_0 \otimes \frac{\lambda_{\text{SOC}}}{2} \begin{pmatrix} 0 & -i & 0 & 0 & 0 & 1 \\ i & 0 & 0 & 0 & 0 & -i \\ 0 & 0 & 0 & -1 & i & 0 \\ 0 & 0 & -1 & 0 & i & 0 \\ 0 & 0 & -i & -i & 0 & 0 \\ 1 & i & 0 & 0 & 0 & 0 \end{pmatrix} \tag{S66}$$

These matrices only have non-zero elements within each sublattice ($A$ or $B$) because the SOC is purely on-site. Finally, the total $p$-orbital tight-binding Hamiltonian consists of both the hopping terms and the on-site SOC contribution,

$$H^{\mathbf{k}}_{p} = H^{\mathbf{k}}_{h} + H_{\text{SOC}} \tag{S67}$$

Below, we explicitly calculate all the hopping matrices defined in Eq. S59 analytically by the Slater-Koster parametrization. Given the directional cosines that characterize the relative orientation between two atoms, the $pp$-hopping matrices can be expressed as

$$t_{pp}(\boldsymbol{n}) = \begin{pmatrix} t_{z,z}(\boldsymbol{n}) & t_{z,x}(\boldsymbol{n}) & t_{z,y}(\boldsymbol{n}) \\ t_{x,z}(\boldsymbol{n}) & t_{x,x}(\boldsymbol{n}) & t_{x,y}(\boldsymbol{n}) \\ t_{y,z}(\boldsymbol{n}) & t_{y,x}(\boldsymbol{n}) & t_{y,y}(\boldsymbol{n}) \end{pmatrix} \tag{S68}$$

Similarly, the $pd$-hopping matrices, which depend on the directional cosines of the bond connecting the two atoms, are given by

$$t_{pd}(\boldsymbol{n}) = \left(t_{z,z^2}(\boldsymbol{n}), t_{x,z^2}(\boldsymbol{n}), t_{y,z^2}(\boldsymbol{n})\right) \tag{S69}$$

For first-nearest $pd$ hoppings occurring via the upper layer of the original A sublattice, the hopping matrices are given by

$$t_{pd}(R_1^+) = \left(-\sin\delta, \frac{\sqrt{3}}{2}\cos\delta, \frac{1}{2}\cos\delta\right), \quad t_{pd}(R_2^+) = \left(-\sin\delta, -\frac{\sqrt{3}}{2}\cos\delta, \frac{1}{2}\cos\delta\right), \quad t_{pd}(R_3^+) = (-\sin\delta, 0, -\cos\delta) \tag{S70}$$

$$t_{pd}(L_1^+) = \left(\sin\delta, -\frac{\sqrt{3}}{2}\cos\delta, -\frac{1}{2}\cos\delta\right), \quad t_{pd}(L_2^+) = \left(\sin\delta, \frac{\sqrt{3}}{2}\cos\delta, -\frac{1}{2}\cos\delta\right), \quad t_{pd}(L_3^+) = (\sin\delta, 0, \cos\delta) \tag{S71}$$

Similarly, for first-nearest $pd$ hoppings via the lower layer of the original A sublattice, the corresponding hopping matrices are obtained by replacing $\delta$ with $-\delta$:

$$t_{pd}(R_1^-) = \left(\sin\delta, \frac{\sqrt{3}}{2}\cos\delta, \frac{1}{2}\cos\delta\right), \quad t_{pd}(R_2^-) = \left(\sin\delta, -\frac{\sqrt{3}}{2}\cos\delta, \frac{1}{2}\cos\delta\right), \quad t_{pd}(R_3^-) = (\sin\delta, 0, -\cos\delta) \tag{S72}$$

$$t_{pd}(L_1^-) = \left(-\sin\delta, -\frac{\sqrt{3}}{2}\cos\delta, -\frac{1}{2}\cos\delta\right), \quad t_{pd}(L_2^-) = \left(-\sin\delta, \frac{\sqrt{3}}{2}\cos\delta, -\frac{1}{2}\cos\delta\right), \quad t_{pd}(L_3^-) = (-\sin\delta, 0, \cos\delta) \tag{S73}$$

Including the second-order correction of the $pd$-hopping parameters, we now present the calculated first-nearest neighbor $pp$-hopping matrices. For instance, we use the notation $t^{AB\uparrow}_{\Delta\mathbf{R}(0,0,0)}$ to denote the hopping of a spin-up electron from a tellurium atom on sublattice A to a tellurium atom on sublattice B between unit cells with no translation (i.e., $\Delta\mathbf{R} = (0,0,0)$).

The calculated first-nearest neighbor $pp$ hopping matrices are presented below

$$\begin{aligned} t^{AB\uparrow}_{\Delta\mathbf{R}(0,0,0)} &= t_{pp}(B_3) + \frac{1}{\epsilon} t_{pd}(L_1^+)\, t_{pd}(R_2^+)^T + \frac{1}{\epsilon} t_{pd}(L_2^+)\, t_{pd}(R_1^+)^T \\ &= \begin{pmatrix} (1-c_3)\, V_{1pp\sigma} + c_3 V_{1pp\pi} - 2c_1^+ & 0 & -\rho\left(V_{1pp\sigma} - V_{1pp\pi}\right) + c_1^+ c_2^+ \\ 0 & V_{1pp\pi} + \frac{3}{2}\left(\lambda_+ - c_1^+\right) & 0 \\ -\rho\left(V_{1pp\sigma} - V_{1pp\pi}\right) + c_1^+ c_2^+ & 0 & c_3 V_{1pp\sigma} + (1-c_3)\, V_{1pp\pi} - \frac{1}{2}\left(\lambda_+ - c_1^+\right) \end{pmatrix} \end{aligned} \tag{S74}$$

Here $\varepsilon = \varepsilon_p - \varepsilon_d$. Similarly $t^{AB\downarrow}_{\Delta\mathbf{R}(0,0,0)}$ can be obtained by replacing the antiferromagnetic index of the Slater-Koster parameters $+ \to -$. $t^{BA\uparrow}_{\Delta\mathbf{R}(0,0,1)}$ and $t^{BA\downarrow}_{\Delta\mathbf{R}(0,0,1)}$ can be obtained by copying as $t^{AB\downarrow}_{\Delta\mathbf{R}(0,0,0)}$ and $t^{AB\uparrow}_{\Delta\mathbf{R}(0,0,0)}$, respectively, and flipping the sign of the matrix elements of $t_{xy}, t_{xz}, t_{yx}, t_{zx}$.

$$\begin{aligned} t^{AB\uparrow}_{\Delta\mathbf{R}(-1,0,0)} &= t_{pp}(B_2) + \frac{1}{\epsilon} t_{pd}(L_1^+)\, t_{pd}(R_3^+)^T + \frac{1}{\epsilon} t_{pd}(L_3^+)\, t_{pd}(R_1^+)^T \\ &= \begin{pmatrix} (1-c_3)\, V_{1pp\sigma} + c_3 V_{1pp\pi} - 2c_1^+ & -\frac{\sqrt{3}}{2}\rho\left(V_{1pp\sigma} - V_{1pp\pi}\right) + \frac{\sqrt{3}}{2}c_1^+ c_2^+ & \frac{1}{2}\rho\left(V_{1pp\sigma} - V_{1pp\pi}\right) - \frac{1}{2}c_1^+ c_2^+ \\ -\frac{\sqrt{3}}{2}\rho\left(V_{1pp\sigma} - V_{1pp\pi}\right) + \frac{\sqrt{3}}{2}c_1^+ c_2^+ & \frac{3}{4}c_3 V_{1pp\sigma} + \left(1 - \frac{3}{4}c_3\right) V_{1pp\pi} & -\frac{\sqrt{3}}{4}c_3\left(V_{1pp\sigma} - V_{1pp\pi}\right) + \frac{\sqrt{3}}{2}\left(\lambda_+ - c_1^+\right) \\ \frac{1}{2}\rho\left(V_{1pp\sigma} - V_{1pp\pi}\right) - \frac{1}{2}c_1^+ c_2^+ & -\frac{\sqrt{3}}{4}c_3\left(V_{1pp\sigma} - V_{1pp\pi}\right) + \frac{\sqrt{3}}{2}\left(\lambda_+ - c_1^+\right) & \frac{1}{4}c_3 V_{1pp\sigma} + \left(1 - \frac{1}{4}c_3\right) V_{1pp\pi} + \lambda_+ - c_1^+ \end{pmatrix} \end{aligned} \tag{S75}$$

$t^{AB\downarrow}_{\Delta\mathbf{R}(-1,0,0)}$ can be obtained by replacing the antiferromagnetic index of the Slater-Koster parameters $+ \to -$. $t^{BA\uparrow}_{\Delta\mathbf{R}(1,0,1)}$ and $t^{BA\downarrow}_{\Delta\mathbf{R}(1,0,1)}$ can be obtained by copying as $t^{AB\downarrow}_{\Delta\mathbf{R}(-1,0,0)}$ and $t^{AB\uparrow}_{\Delta\mathbf{R}(-1,0,0)}$, respectively, and flipping the sign of the matrix elements of $t_{xy}, t_{xz}, t_{yx}, t_{zx}$.

$$\begin{aligned} t^{AB\uparrow}_{\Delta\mathbf{R}(0,1,0)} &= t_{pp}(B_1) + \frac{1}{\epsilon} t_{pd}(L_2^+)\, t_{pd}(R_3^+)^T + \frac{1}{\epsilon} t_{pd}(L_3^+)\, t_{pd}(R_2^+)^T \\ &= \begin{pmatrix} (1-c_3)\, V_{1pp\sigma} + c_3 V_{1pp\pi} - 2c_1^+ & \frac{\sqrt{3}}{2}\rho\left(V_{1pp\sigma} - V_{1pp\pi}\right) - \frac{\sqrt{3}}{2}c_1^+ c_2^+ & \frac{1}{2}\rho\left(V_{1pp\sigma} - V_{1pp\pi}\right) - \frac{1}{2}c_1^+ c_2^+ \\ \frac{\sqrt{3}}{2}\rho\left(V_{1pp\sigma} - V_{1pp\pi}\right) - \frac{\sqrt{3}}{2}c_1^+ c_2^+ & \frac{3}{4}c_3 V_{1pp\sigma} + \left(1 - \frac{3}{4}c_3\right) V_{1pp\pi} & \frac{\sqrt{3}}{4}c_3\left(V_{1pp\sigma} - V_{1pp\pi}\right) - \frac{\sqrt{3}}{2}\left(\lambda_+ - c_1^+\right) \\ \frac{1}{2}\rho\left(V_{1pp\sigma} - V_{1pp\pi}\right) - \frac{1}{2}c_1^+ c_2^+ & \frac{\sqrt{3}}{4}c_3\left(V_{1pp\sigma} - V_{1pp\pi}\right) - \frac{\sqrt{3}}{2}\left(\lambda_+ - c_1^+\right) & \frac{1}{4}c_3 V_{1pp\sigma} + \left(1 - \frac{1}{4}c_3\right) V_{1pp\pi} + \lambda_+ - c_1^+ \end{pmatrix} \end{aligned} \tag{S76}$$

$t^{AB\downarrow}_{\Delta\mathbf{R}(0,1,0)}$ can be obtained by replacing the antiferromagnetic index of the Slater-Koster parameters $+ \to -$. $t^{BA\uparrow}_{\Delta\mathbf{R}(0,-1,1)}$ and $t^{BA\downarrow}_{R(0,-1,1)}$ can be obtained by copying as $t^{AB\downarrow}_{\Delta\mathbf{R}(0,1,0)}$ and $t^{AB\uparrow}_{\Delta\mathbf{R}(0,1,0)}$, respectively, and flipping the sign of the matrix elements of $t_{xy}, t_{xz}, t_{yx}, t_{zx}$.

The calculated second-nearest neighbor $pp$ hopping matrices are presented below

$$
\begin{aligned}
t^{AA\uparrow}_{R(1,0,0)} &= t_{pp}(S_3) + \frac{1}{\epsilon} t_{pd}(R_3^+)\, t_{pd}(R_2^+)^T + \frac{1}{\epsilon} t_{pd}(R_3^-)\, t_{pd}(R_2^-)^T \\
&= \begin{pmatrix} V_{2pp\pi} + g_1 & 0 & g_2^+ \\ \frac{\sqrt{3}}{2} g_2^+ & \frac{1}{4} V_{2pp\sigma} + \frac{3}{4} V_{2pp\pi} & -\frac{\sqrt{3}}{4}\left(V_{2pp\sigma} - V_{2pp\pi}\right) + \frac{\sqrt{3}}{2}\left(\lambda_g - g_1\right) \\ -\frac{1}{2} g_2^+ & -\frac{\sqrt{3}}{4}\left(V_{2pp\sigma} - V_{2pp\pi}\right) & \frac{3}{4} V_{2pp\sigma} + \frac{1}{4} V_{2pp\pi} - \frac{1}{2}\left(\lambda_g - g_1\right) \end{pmatrix}
\end{aligned}
\tag{S77}
$$

$t^{AA\downarrow}_{R(1,0,0)}$ can be obtained by replacing the antiferromagnetic index of the Slater-Koster parameters $+ \to -$ and by flipping the sign of the matrix elements of $t_{xy}, t_{xz}, t_{yx}, t_{zx}$. $t^{BB\uparrow}_{R(-1,0,1)}$ and $t^{BB\downarrow}_{R(-1,0,1)}$ can be obtained by transposing $t^{AA\downarrow}_{R(1,0,0)}$ and $t^{AA\uparrow}_{R(1,0,0)}$, respectively.

$$
\begin{aligned}
t^{AA\uparrow}_{R(1,1,0)} &= t_{pp}(S_2) + \frac{1}{\epsilon} t_{pd}(R_1^+)\, t_{pd}(R_2^+)^T + \frac{1}{\epsilon} t_{pd}(R_1^-)\, t_{pd}(R_2^-)^T \\
&= \begin{pmatrix} V_{2pp\pi} + g_1 & -\frac{\sqrt{3}}{2} g_2^+ & -\frac{1}{2} g_2^+ \\ \frac{\sqrt{3}}{2} g_2^+ & V_{2pp\sigma} - \frac{3}{4}\left(\lambda_g - g_1\right) & -\frac{\sqrt{3}}{4}\left(\lambda_g - g_1\right) \\ -\frac{1}{2} g_2^+ & \frac{\sqrt{3}}{4}\left(\lambda_g - g_1\right) & V_{2pp\pi} + \frac{1}{4}\left(\lambda_g - g_1\right) \end{pmatrix}
\end{aligned}
\tag{S78}
$$

$t^{AA\downarrow}_{R(1,1,0)}$ can be obtained by replacing the antiferromagnetic index of the Slater-Koster parameters $+ \to -$ and by flipping the sign of the matrix elements of $t_{xy}, t_{xz}, t_{yx}, t_{zx}$. $t^{BB\uparrow}_{R(-1,-1,1)}$ and $t^{BB\downarrow}_{R(-1,-1,1)}$ can be obtained by transposing $t^{AA\downarrow}_{R(1,1,0)}$ and $t^{AA\uparrow}_{R(1,1,0)}$, respectively.

$$
\begin{aligned}
t^{AA\uparrow}_{R(0,1,0)} &= t_{pp}(S_1) + \frac{1}{\epsilon} t_{pd}(R_1^+)\, t_{pd}(R_3^+)^T + \frac{1}{\epsilon} t_{pd}(R_1^-)\, t_{pd}(R_3^-)^T \\
&= \begin{pmatrix} V_{2pp\pi} + g_1 & -\frac{\sqrt{3}}{2} g_2^+ & -\frac{1}{2} g_2^+ \\ 0 & \frac{1}{4} V_{2pp\sigma} + \frac{3}{4} V_{2pp\pi} & \frac{\sqrt{3}}{4}\left(V_{2pp\sigma} - V_{2pp\pi}\right) \\ g_2^+ & \frac{\sqrt{3}}{4}\left(V_{2pp\sigma} - V_{2pp\pi}\right) - \frac{\sqrt{3}}{2}\left(\lambda_g - g_1\right) & \frac{3}{4} V_{2pp\sigma} + \frac{1}{4} V_{2pp\pi} - \frac{1}{2}\left(\lambda_g - g_1\right) \end{pmatrix}
\end{aligned}
\tag{S79}
$$

$t^{AA\downarrow}_{R(0,1,0)}$ can be obtained by replacing the antiferromagnetic index of the Slater-Koster parameters $+ \to -$ and by flipping the sign of the matrix elements of $t_{xy}, t_{xz}, t_{yx}, t_{zx}$. $t^{BB\uparrow}_{R(0,-1,1)}$ and $t^{BB\downarrow}_{R(0,-1,1)}$ can be obtained by transposing $t^{AA\downarrow}_{R(0,1,0)}$ and $t^{AA\uparrow}_{R(0,1,0)}$, respectively. The calculated third-nearest neighbor $pp$ hopping matrices are presented below

$$
t^{AB\uparrow}_{R(-1,-1,0)} = t_{pp}(R_1^+) + \frac{1}{\epsilon} t_{pd}(L_1^+)\, t_{pd}(R_1^+)^T =
$$
$$
\begin{pmatrix} (1 - c_4)\, V^+_{3pp\sigma} + c_4 V^+_{3pp\pi} - c_1^+ & -\frac{\sqrt{3}}{2}\chi\left(V^+_{3pp\sigma} - V^+_{3pp\pi}\right) + \frac{\sqrt{3}}{2} c_1^+ c_2^+ & -\frac{1}{2}\chi\left(V^+_{3pp\sigma} - V^+_{3pp\pi}\right) + \frac{1}{2} c_1^+ c_2^+ \\ -\frac{\sqrt{3}}{2}\chi\left(V^+_{3pp\sigma} - V^+_{3pp\pi}\right) + \frac{\sqrt{3}}{2} c_1^+ c_2^+ & \frac{3}{4} c_4 V^+_{3pp\sigma} + \left(1 - \frac{3}{4} c_4\right) V^+_{3pp\pi} - \frac{3}{4}\left(\lambda_+ - c_1^+\right) & \frac{\sqrt{3}}{4} c_4 \left(V^+_{3pp\sigma} - V^+_{3pp\pi}\right) - \frac{\sqrt{3}}{4}\left(\lambda_+ - c_1^+\right) \\ -\frac{1}{2}\chi\left(V^+_{3pp\sigma} - V^+_{3pp\pi}\right) + \frac{1}{2} c_1^+ c_2^+ & \frac{\sqrt{3}}{4} c_4 \left(V^+_{3pp\sigma} - V^+_{3pp\pi}\right) - \frac{\sqrt{3}}{4}\left(\lambda_+ - c_1^+\right) & \frac{1}{4} c_4 V^+_{3pp\sigma} + \left(1 - \frac{1}{4} c_4\right) V^+_{3pp\pi} - \frac{1}{4}\left(\lambda_+ - c_1^+\right) \end{pmatrix}
\tag{S80}
$$

and $t^{AB\downarrow}_{R(-1,-1,0)}$ can be obtained by replacing the antiferromagnetic index of the Slater-Koster parameters $+ \to -$. $t^{BA\uparrow}_{R(1,1,1)}$ and $t^{BA\downarrow}_{R(1,1,1)}$ can be obtained by copying as $t^{AB\downarrow}_{R(-1,-1,0)}$ and $t^{AB\uparrow}_{R(-1,-1,0)}$, respectively, and flipping the sign of the matrix elements of $t_{xy}, t_{xz}, t_{yx}, t_{zx}$.

$$
t^{AB\uparrow}_{R(1,1,0)} = t_{pp}(R_2^+) + \frac{1}{\epsilon} t_{pd}(L_2^+)\, t_{pd}(R_2^+)^T =
$$
$$
\begin{pmatrix} (1 - c_4)\, V^+_{3pp\sigma} + c_4 V^+_{3pp\pi} - c_1^+ & \frac{\sqrt{3}}{2}\chi\left(V^+_{3pp\sigma} - V^+_{3pp\pi}\right) - \frac{\sqrt{3}}{2} c_1^+ c_2^+ & -\frac{1}{2}\chi\left(V^+_{3pp\sigma} - V^+_{3pp\pi}\right) + \frac{1}{2} c_1^+ c_2^+ \\ \frac{\sqrt{3}}{2}\chi\left(V^+_{3pp\sigma} - V^+_{3pp\pi}\right) - \frac{\sqrt{3}}{2} c_1^+ c_2^+ & \frac{3}{4} c_4 V^+_{3pp\sigma} + \left(1 - \frac{3}{4} c_4\right) V^+_{3pp\pi} - \frac{3}{4}\left(\lambda_+ - c_1^+\right) & -\frac{\sqrt{3}}{4} c_4 \left(V^+_{3pp\sigma} - V^+_{3pp\pi}\right) + \frac{\sqrt{3}}{4}\left(\lambda_+ - c_1^+\right) \\ -\frac{1}{2}\chi\left(V^+_{3pp\sigma} - V^+_{3pp\pi}\right) + \frac{1}{2} c_1^+ c_2^+ & -\frac{\sqrt{3}}{4} c_4 \left(V^+_{3pp\sigma} - V^+_{3pp\pi}\right) + \frac{\sqrt{3}}{4}\left(\lambda_+ - c_1^+\right) & \frac{1}{4} c_4 V^+_{3pp\sigma} + \left(1 - \frac{1}{4} c_4\right) V^+_{3pp\pi} - \frac{1}{4}\left(\lambda_+ - c_1^+\right) \end{pmatrix}
\tag{S81}
$$

and $t^{AB\downarrow}_{R(1,1,0)}$ can be obtained by replacing the antiferromagnetic index of the Slater-Koster parameters $+ \to -$. $t^{BA\uparrow}_{R(-1,-1,1)}$ and $t^{BA\downarrow}_{R(-1,-1,1)}$ can be obtained by copying as $t^{AB\downarrow}_{R(1,1,0)}$ and $t^{AB\uparrow}_{R(1,1,0)}$, respectively, and flipping the sign of the matrix elements of

$t_{xy}, t_{xz}, t_{yx}, t_{zx}$.

$$t^{AB\uparrow}_{R(-1,1,0)} = t_{pp}(R^+_3) + \frac{1}{\epsilon} t_{pd}(L^+_3)\, t_{pd}(R^+_3)^T =$$
$$\begin{pmatrix} (1-c_4)\, V^+_{3pp\sigma} + c_4 V^+_{3pp\pi} - c^+_1 & 0 & \chi\left(V^+_{3pp\sigma} - V^+_{3pp\pi}\right) - c^+_1 c^+_2 \\ 0 & V^+_{3pp\pi} & 0 \\ \chi\left(V^+_{3pp\sigma} - V^+_{3pp\pi}\right) - c^+_1 c^+_2 & 0 & c_4 V^+_{3pp\sigma} + (1-c_4)\, V^+_{3pp\pi} - \left(\lambda_+ - c^+_1\right) \end{pmatrix} \tag{S82}$$

and $t^{AB\downarrow}_{R(-1,1,0)}$ can be obtained by replacing the antiferromagnetic index of the Slater-Koster parameters $+ \to -$. $t^{BA\uparrow}_{R(1,-1,1)}$ and $t^{BA\downarrow}_{R(1,-1,1)}$ can be obtained by copying as $t^{AB\downarrow}_{R(-1,1,0)}$ and $t^{AB\uparrow}_{R(-1,1,0)}$, respectively, and flipping the sign of the matrix elements of $t_{xy}, t_{xz}, t_{yx}, t_{zx}$.

From the above, we have calculated all the $p$-orbital hopping matrices explicitly, including $d$-orbital mediated hopping contributions.

## V. OBTAINING NUMERICAL VALUES FOR SK PARAMETERS BY FITTING TO DFT WANNIER MATRICES

As derived in the previous chapter, we obtained analytical expressions for the matrix elements of the hopping Hamiltonian in terms of our Slater–Koster parameters. For the lattice constants, we adopted the experimental values $a = 4.171$Å and $c = 6.686$Å [3]. In the fitting procedure, these analytical expressions are equated to the corresponding numerical matrix elements extracted from the DFT Wannier matrices, yielding a system of algebraic equations. By solving these equations, we extract the best-fit values for the parameters for Eq. S56. The fitted values are:

$$\begin{aligned} V_{1pp\sigma} &= 0.535 \text{ eV}, \quad V_{1pp\pi} = -0.019 \text{ eV}, \quad V_{2pp\sigma} = 0.438 \text{ eV}, \quad V_{2pp\pi} = 0.0260 \text{ eV} \\ V^+_{3pp\sigma} &= 0.110 \text{ eV}, \quad V^+_{3pp\pi} = 0.0267 \text{ eV}, \quad V^-_{3pp\sigma} = -0.286 \text{ eV}, \quad V^-_{3pp\pi} = -0.0120 \text{ eV} \\ c^+_1 &= -0.0276 \text{ eV}, \quad c^+_2 = 1.175 \text{ eV}, \quad c^-_1 = -0.0594 \text{ eV}, \quad c^-_2 = 1.353 \text{ eV} \\ \lambda_+ &= -0.0522 \text{ eV}, \quad \lambda_- = -0.192 \text{ eV}, \quad \epsilon_x = 3.05 \text{ eV}, \quad \epsilon_y = 3.05 \text{ eV}, \quad \epsilon_z = 2.99 \text{ eV} \\ \lambda_{\text{SOC}} &= 0.44 \text{ eV} \end{aligned} \tag{S83}$$

Using these fitted parameters, we diagonalized the Hamiltonian along the high-symmetry path in the Brillouin zone. The resulting band structure, shown in Fig. S3, qualitatively reproduces the DFT band structure below the Fermi surface—which is dominated by $p$-orbitals.

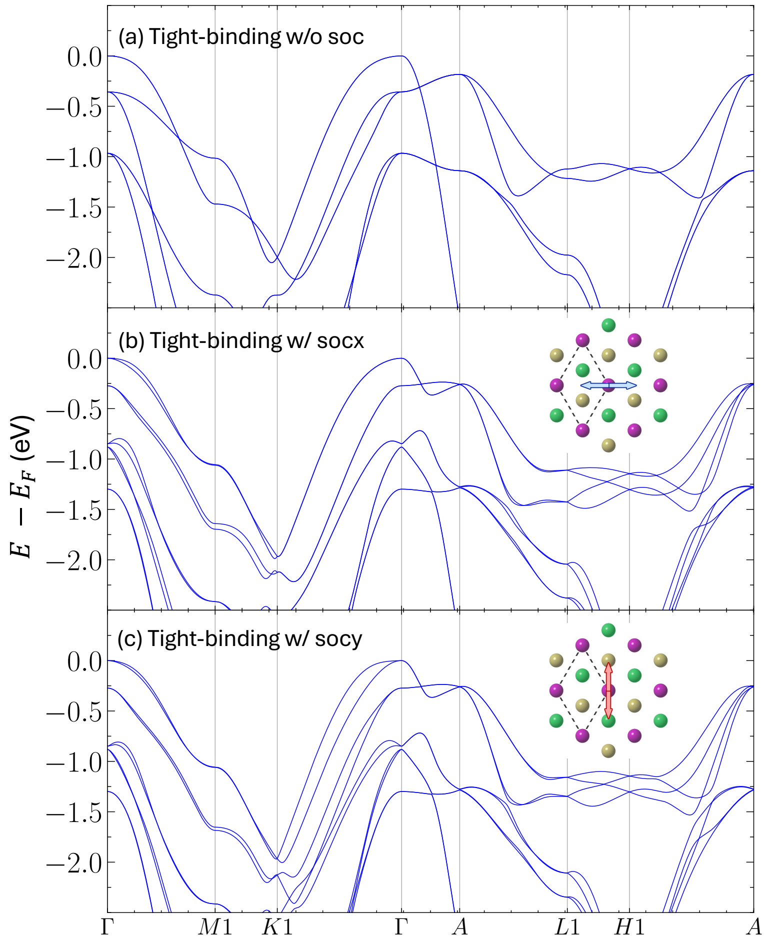


Figure S3. Energy band structures of MnTe calculated from the tight-binding Hamiltonian. The numerical parameters used in these calculations are provided in Eq. S83. Panel (a) shows the bands without spin–orbit coupling (SOC) along the same high-symmetry path as in Fig. 2 in the main text. Panel (b) displays the bands with SOC when the Néel vector is aligned along the $[11\bar{2}0]$ ($x$) direction, and panel (c) shows the corresponding bands with the Néel vector along the $[1\bar{1}00]$ ($y$) direction. These results qualitatively reproduce the DFT findings, with degeneracies protected by the intrinsic symmetry of MnTe.

## VI. EIGENSTATES OF THE $p$-ORBITAL TIGHT-BINDING HAMILTONIAN WITHOUT SOC AT THE Γ AND $A$ POINTS

Here, the complete $p$-orbital Hamiltonian is given by

$$H_p^{\mathbf{k}} = H_h^{\mathbf{k}} + H_{\mathrm{SOC}} \tag{S84}$$

with all matrix elements expressed analytically in terms of the Slater–Koster parameters (see previous chapter). In the absence of SOC, we verified analytically that $H_h^{\mathbf{k}}$ can be diagonalized by an appropriate basis rotation at both the Γ and $A$ points.

At the Γ point, the eigenstates of $H_h^{\mathbf{k}=\Gamma}$ arise from symmetrized and anti-symmetrized combinations of the $p_x$, $p_y$, and $p_z$ orbitals in both the spin-up and spin-down channels (with spin quantized along the $z$-axis). Here, our definition of the symmetrized and anti-symmetrized states of $p_n$ orbitals ($n = x, y, z$) with spin $\sigma$, $|S_n\sigma\rangle$ and $|A_n\sigma\rangle$ respectively, are given by

$$|S_n\sigma\rangle = \frac{1}{\sqrt{2}}\left(|p_{n\sigma}^A\rangle + |p_{n\sigma}^B\rangle\right) \tag{S85}$$

$$|A_n\sigma\rangle = \frac{1}{\sqrt{2}}\left(|p_{n\sigma}^A\rangle - |p_{n\sigma}^B\rangle\right) \tag{S86}$$

The complete set of twelve eigenstates obtained from the tight-binding calculation is listed below. Using the parameter sets in Eq. S83, we find that the highest-energy, two-fold degenerate eigenstates at the Γ point are given by

$$|S_z \uparrow\rangle = \frac{1}{\sqrt{2}}\left(|p^A_{z\uparrow}\rangle + |p^B_{z\uparrow}\rangle\right) \tag{S87}$$

$$|S_z \downarrow\rangle = \frac{1}{\sqrt{2}}\left(|p^A_{z\downarrow}\rangle + |p^B_{z\downarrow}\rangle\right) \tag{S88}$$

These states represent the symmetrized combinations of the $p_z$ orbitals for both spin channels. Notably, these eigenstates, which are located near the Fermi surface, remain spin-degenerate in the absence of SOC. In the absence of SOC, we found that the two-fold degeneracy is protected by symmetry, as confirmed by our group theory analysis. In the next chapter, we derive the effective Hamiltonian around the Γ point by projecting onto this two-dimensional subspace.

We obtained the four-fold degenerate eigenstates with the second highest energy at the Γ point:

$$|S_x \uparrow\rangle = \frac{1}{\sqrt{2}}\left(|p^A_{x\uparrow}\rangle + |p^B_{x\uparrow}\rangle\right) \tag{S89}$$

$$|S_x \downarrow\rangle = \frac{1}{\sqrt{2}}\left(|p^A_{x\downarrow}\rangle + |p^B_{x\downarrow}\rangle\right) \tag{S90}$$

$$|S_y \uparrow\rangle = \frac{1}{\sqrt{2}}\left(|p^A_{y\uparrow}\rangle + |p^B_{y\uparrow}\rangle\right) \tag{S91}$$

$$|S_y \downarrow\rangle = \frac{1}{\sqrt{2}}\left(|p^A_{y\downarrow}\rangle + |p^B_{y\downarrow}\rangle\right) \tag{S92}$$

These states represent the symmetrized combinations of the $p_x$ and $p_y$ orbitals for both spin channels (with spin quantization along the $z$-axis).

Next, we obtained the four-fold degenerate eigenstates with the third highest energy at the Γ point:

$$|A_x \uparrow\rangle = \frac{1}{\sqrt{2}}\left(|p^A_{x\uparrow}\rangle - |p^B_{x\uparrow}\rangle\right) \tag{S93}$$

$$|A_x \downarrow\rangle = \frac{1}{\sqrt{2}}\left(|p^A_{x\downarrow}\rangle - |p^B_{x\downarrow}\rangle\right) \tag{S94}$$

$$|A_y \uparrow\rangle = \frac{1}{\sqrt{2}}\left(|p^A_{y\uparrow}\rangle - |p^B_{y\uparrow}\rangle\right) \tag{S95}$$

$$|A_y \downarrow\rangle = \frac{1}{\sqrt{2}}\left(|p^A_{y\downarrow}\rangle - |p^B_{y\downarrow}\rangle\right) \tag{S96}$$

These correspond to the anti-symmetrized combinations of the $p_x$ and $p_y$ orbitals for both spin-up and spin-down electrons.

Finally, the two-fold degenerate eigenstates with the fourth highest energy at the Γ point are given by:

$$|A_z \uparrow\rangle = \frac{1}{\sqrt{2}}\left(|p^A_{z\uparrow}\rangle - |p^B_{z\uparrow}\rangle\right) \tag{S97}$$

$$|A_z \downarrow\rangle = \frac{1}{\sqrt{2}}\left(|p^A_{z\downarrow}\rangle - |p^B_{z\downarrow}\rangle\right) \tag{S98}$$

These are the anti-symmetrized combinations of the $p_z$ orbitals for both spin channels (with spin quantization along the $z$-axis).

At the $A$ point, the eigenstates of $H_h^{\mathbf{k}=A}$ also arise from symmetrized and anti-symmetrized combinations of the $p_x$, $p_y$, and $p_z$ orbitals in both the spin-up and spin-down channels (with spin quantized along the Néel vector). The complete set of twelve eigenstates obtained from the tight-binding calculation is listed below. Using the parameter sets in Eq. S83, we find that the highest-energy, four-fold degenerate eigenstates at the $A$ point are given by

$$|S_x \uparrow\rangle = \frac{1}{\sqrt{2}}\left(|p^A_{x\uparrow}\rangle + |p^B_{x\uparrow}\rangle\right) \tag{S99}$$

$$|A_x \downarrow\rangle = \frac{1}{\sqrt{2}}\left(|p^A_{x\downarrow}\rangle - |p^B_{x\downarrow}\rangle\right) \tag{S100}$$

$$|S_y \uparrow\rangle = \frac{1}{\sqrt{2}}\left(|p^A_{y\uparrow}\rangle + |p^B_{y\uparrow}\rangle\right) \tag{S101}$$

$$|A_y \downarrow\rangle = \frac{1}{\sqrt{2}}\left(|p^A_{y\downarrow}\rangle - |p^B_{y\downarrow}\rangle\right) \tag{S102}$$

These states correspond, respectively, to the symmetrized combination of the $p_x$ orbital (spin up), the anti-symmetrized combination of the $p_x$ orbital (spin down), the symmetrized combination of the $p_y$ orbital (spin up), and the anti-symmetrized combination of the $p_y$ orbital (spin down). Notably, these eigenstates, which lie near the Fermi surface, exhibit the characteristic $A/B$ sublattice pseudospin splitting. In the absence of SOC, we found that the four-fold degeneracy is protected by symmetry, as confirmed by our group theory analysis. In the next chapter, we derive the effective Hamiltonian around the $A$ point by projecting onto this four-dimensional subspace.

We obtained the four-fold degenerate eigenstates with the second highest energy at the $A$ point:

$$|A_x \uparrow\rangle = \frac{1}{\sqrt{2}}\left(|p^A_{x\uparrow}\rangle - |p^B_{x\uparrow}\rangle\right) \tag{S103}$$

$$|S_x \downarrow\rangle = \frac{1}{\sqrt{2}}\left(|p^A_{x\downarrow}\rangle + |p^B_{x\downarrow}\rangle\right) \tag{S104}$$

$$|A_y \uparrow\rangle = \frac{1}{\sqrt{2}}\left(|p^A_{y\uparrow}\rangle - |p^B_{y\uparrow}\rangle\right) \tag{S105}$$

$$|S_y \downarrow\rangle = \frac{1}{\sqrt{2}}\left(|p^A_{y\downarrow}\rangle + |p^B_{y\downarrow}\rangle\right) \tag{S106}$$

These states correspond respectively to the anti-symmetrized $p_x$ orbital with spin up, the symmetrized $p_x$ orbital with spin down, the anti-symmetrized $p_y$ orbital with spin up, and the symmetrized $p_y$ orbital with spin down. They represent the pseudospin-split counterparts of the four-fold degenerate $p_x$ and $p_y$ states.

Next, we obtained the two-fold degenerate eigenstates with the third highest energy at the $A$ point:

$$|S_z \uparrow\rangle = \frac{1}{\sqrt{2}}\left(|p^A_{z\uparrow}\rangle + |p^B_{z\uparrow}\rangle\right) \tag{S107}$$

$$|A_z \downarrow\rangle = \frac{1}{\sqrt{2}}\left(|p^A_{z\downarrow}\rangle - |p^B_{z\downarrow}\rangle\right) \tag{S108}$$

These correspond respectively to the symmetrized state of the $p_z$ orbital with spin up and the anti-symmetrized state of the $p_z$ orbital with spin down. These $p_z$ eigenstates exhibit the $A/B$ sublattice pseudospin-splitting, similar to the splitting observed in the $p_x$ and $p_y$ orbital cases.

Finally, the two-fold degenerate eigenstates with the fourth highest energy at the $A$ point are given by:

$$|A_z \uparrow\rangle = \frac{1}{\sqrt{2}}\left(|p^A_{z\uparrow}\rangle - |p^B_{z\uparrow}\rangle\right) \tag{S109}$$

$$|S_z \downarrow\rangle = \frac{1}{\sqrt{2}}\left(|p^A_{z\downarrow}\rangle + |p^B_{z\downarrow}\rangle\right) \tag{S110}$$

These correspond, respectively, to the anti-symmetrized state of the $p_z$ orbital with spin up and the symmetrized state of the $p_z$ orbital with spin down. They represent the pseudospin-split counterparts of the two-fold degenerate $p_z$ states.

Above, we have listed all the exactly diagonalized eigenstates of $H_h^{\mathbf{k}=\Gamma}$ and $H_h^{\mathbf{k}=A}$. By transforming the tight-binding Hamiltonian into these bases at the $\Gamma$ and $A$ points, the off-diagonal matrix elements vanish at these high-symmetry points (except for those arising from $H_{\text{SOC}}$, and become $\mathbf{k}$-dependent. Consequently, the coupling between the effective Hamiltonian subspace and its orthogonal complement can be treated as a perturbation. In the next chapter, we detail the derivation of the effective Hamiltonian via a second-order canonical transformation that preserves the symmetry of MnTe.

## VII. SECOND-ORDER CANONICAL TRANSFORMATION AND DERIVING EFFECTIVE HAMILTONIAN

Using the tight-binding Hamiltonian above, we can now project the full $p$-orbital Hamiltonian $H_p^{\mathbf{k}}$ onto the relevant orbitals by further application of the Schrieffer-Wolff transformation [4, 5], and expand the effective Hamiltonian around corresponding high symmetric point in the Brillouin zone. The $p$-orbital Hamiltonian can be regrouped as the following.

$$H_p^{\mathbf{k}} = \begin{pmatrix} H^H & V \\ V^\dagger & H^L \end{pmatrix} \tag{S111}$$

where $H^H$ is the matrix representation of the Hamiltonian in the subspace spanned by the basis for effective Hamiltonian, while $H^L$ is the matrix representation of the Hamiltonian in the subspace spanned by the other orthogonal basis. $V$ is the matrix describing the hopping between these two subspaces, and this part should be integrated out by the canonical transformation we employ up to the second order of $V/\left(\Lambda^H - H^L\right)$. Here, $\Lambda^H$ and $\Lambda^L$ are diagonal components of $H^H$ and $H^L$ respectively. Then, the second-order Schrieffer-Wolff transformation is given by

$$H_{\text{eff}} = H^H + \Delta H \tag{S112}$$

where

$$\Delta H = V\left(\Lambda^H - H^L\right)^{-1} V^\dagger = V\left[\left(\Lambda^H - \Lambda^L\right)\{1 - \left(\Lambda^H - \Lambda^L\right)^{-1}\left(H^L - \Lambda^L\right)\}\right]^{-1} V^\dagger \tag{S113}$$

$$= V\left[1 - \left(\Lambda^H - \Lambda^L\right)^{-1}\left(H^L - \Lambda^L\right)\right]^{-1}\left(\Lambda^H - \Lambda^L\right)^{-1} V^\dagger \tag{S114}$$

$$= V\left(\Lambda^H - \Lambda^L\right)^{-1} V^\dagger + V\left(\Lambda^H - \Lambda^L\right)^{-1}\left(H^L - \Lambda^L\right)\left(\Lambda^H - \Lambda^L\right)^{-1} V^\dagger + O\left(\left[\left(\Lambda^H - \Lambda^L\right)^{-1}\left(H^L - \Lambda^L\right)\right]^2\right) \tag{S115}$$

Note that the matrix elements in $\left(\Lambda^H - \Lambda^L\right)^{-1}$ are independent of $\mathbf{k}$, and other matrix elements in $V$ and $\left(H^L - \Lambda^L\right)$ are at least first order in $\mathbf{k}$, with the exception of the SOC terms. Therefore, by retaining terms up to second order in $\mathbf{k}$ with linear SOC, the expression below effectively incorporates all quadratic $\mathbf{k}$ terms with linear SOC, as well as the $\mathbf{k}$-independent contributions arising from quadratic SOC.

$$H_{\text{eff}} = H^H + V\left(\Lambda^H - \Lambda^L\right)^{-1} V^\dagger + V\left(\Lambda^H - \Lambda^L\right)^{-1}\left(H^L - \Lambda^L\right)\left(\Lambda^H - \Lambda^L\right)^{-1} V^\dagger \tag{S116}$$

We found that including the third term in Eq. S116 is essential to capture all quadratic $\mathbf{k}$ terms with linear SOC; omitting it would lead to a spurious violation of the symmetry constraint in Eq. S10.

Note that if one were to derive quintic $\mathbf{k}$ terms or quadratic $\mathbf{k}$ terms with quadratic SOC contributions, a fourth-order canonical transformation would be required. Such higher-order corrections are beyond the scope of the present work.

In the following sections, we apply this projection method to derive effective Hamiltonians around the $\Gamma$ and $A$ points.

### A. Effective Hamiltonian around $A$ point

We start from the non-SOC Hamiltonian. At the $A$ point, $(k_x, k_y, k_z) = (0, 0, \pi/d)$, the basis of the four-fold degenerated bands near the Fermi surface are given by

$$|S_x \uparrow\rangle = \frac{1}{\sqrt{2}}\left(|p^A_{x\uparrow}\rangle + |p^B_{x\uparrow}\rangle\right) \tag{S117}$$

$$|A_x \downarrow\rangle = \frac{1}{\sqrt{2}}\left(|p^A_{x\downarrow}\rangle - |p^B_{x\downarrow}\rangle\right) \tag{S118}$$

$$|S_y \uparrow\rangle = \frac{1}{\sqrt{2}}\left(|p^A_{y\uparrow}\rangle + |p^B_{y\uparrow}\rangle\right) \tag{S119}$$

$$|A_y \downarrow\rangle = \frac{1}{\sqrt{2}}\left(|p^A_{y\downarrow}\rangle - |p^B_{y\downarrow}\rangle\right) \tag{S120}$$

Here, $|S\uparrow\rangle$ refers to a symmetrized state of the sublattice orbitals with spin up, while $|A\downarrow\rangle$ is an anti-symmetrized state with spin down, which is following the definitions in Eqs. S85 and S86. The spin quantization axis is chosen along the Néel vector,

which lies either along [11$\bar{2}$0] (the $x$ direction) or [1$\bar{1}$00] (the $y$ direction). After adding the spin-orbit coupling $H_{\mathrm{SOC}}$, they split into two two-fold degenerated bands, but the width of the splitting is still small compared to the energy difference with other bands. Therefore, we project onto the same sub-Hilbert space with similar canonical transformation using Eq. S116, where $H^H$ is spanned by the four basis listed above (ordered as given).

After performing the canonical transformation, we obtain the effective Hamiltonian for the AFM MnTe without SOC at the $A$ point, derived analytically in the following form:

$$H^A_{\text{non-SOC}} = \left[c_1\left(k_x^2+k_y^2\right)+c_2k_z^2\right](\tau_0\otimes\omega_0)+c_3\left[\left(k_x^2-k_y^2\right)(\tau_z\otimes\omega_0)+2k_xk_y(\tau_x\otimes\omega_0)\right]+c_4\left[k_zk_x(\tau_x\otimes\omega_z)+k_yk_z(\tau_z\otimes\omega_z)\right] \tag{S121}$$

Here, $\boldsymbol{\tau}$ is a pseudospin for $p_x/p_y$ orbitals, $\boldsymbol{\omega}$ is a pseudospin to indicate the two-fold degeneracy between $|S\uparrow\rangle$ and $|A\downarrow\rangle$. $c_{1,2,3,4}$ are independent parameters, which depends on the parameters in Eq. S51 in complicated form. Those terms are all allowed by the symmetry constraints.

Once we add the on-site SOC matrix given by Eq. IV, there appears the correction terms which we derived up to linear order of SOC, in both cases with Néel vector along [11$\bar{2}$0] ($x$) direction, or [1$\bar{1}$00] ($y$) direction.

$$\begin{aligned} H^A_{[11\bar{2}0]} &= H^A_{\text{non-SOC}}+\gamma_0(\tau_z\otimes\omega_0)+\gamma_1\left[k_x(\tau_z\otimes\omega_x)-k_y(\tau_x\otimes\omega_x)\right]+\gamma_2k_y\left(\tau_y\otimes\omega_x\right)\\ &\quad+\gamma_3k_z\left(\tau_y\otimes\omega_y\right)+\gamma_4k_xk_y\left(\tau_y\otimes\omega_0\right)+\gamma_5k_xk_z\left(\tau_y\otimes\omega_z\right) \end{aligned} \tag{S122}$$

$$\begin{aligned} H^A_{[1\bar{1}00]} &= H^A_{\text{non-SOC}}-\gamma_0(\tau_z\otimes\omega_0)+\gamma_1\left(k_x\tau_z-k_y\tau_x\right)\otimes\omega_x-\gamma_2k_x\left(\tau_y\otimes\omega_x\right)\\ &\quad+\gamma_3k_z\left(\tau_y\otimes\omega_y\right)+\frac{\gamma_4}{2}\left(k_x^2-k_y^2\right)\left(\tau_y\otimes\omega_0\right)+\gamma_5k_yk_z\left(\tau_y\otimes\omega_z\right) \end{aligned} \tag{S123}$$

Here, $\gamma_{1,2,3,4,5}$ are independent parameters with linear SOC, which depends on the parameters in Eq. S51 in complicated form. $\gamma_0$ determines the energy gap within the projected subspace, however, it is quadratic SOC and thus negligibly small. We found that all parameters $\gamma_{0,1,2,3,4,5}$ are analytically related between the two cases, as shown in Eqs. S122 and S123. This analytical relationship was further validated by fitting the effective Hamiltonian to the DFT results.

### B. Effective Hamiltonian around Γ point

We begin with the non-SOC Hamiltonian at the Γ point, $(k_x,k_y,k_z)=(0,0,0)$. Here, the two-fold degenerate bands near the Fermi surface are spanned by the following symmetrized combinations of $p_z$ orbitals:

$$|S_z\uparrow\rangle = \frac{1}{\sqrt{2}}\left(|p^A_{z\uparrow}\rangle+|p^B_{z\uparrow}\rangle\right) \tag{S124}$$

$$|S_z\downarrow\rangle = \frac{1}{\sqrt{2}}\left(|p^A_{z\downarrow}\rangle+|p^B_{z\downarrow}\rangle\right) \tag{S125}$$

with the spin quantization axis along the $z$ axis. These states serve as the relevant subspace for constructing the effective Hamiltonian at Γ, regardless of whether the Néel vector lies along [11$\bar{2}$0] ($x$) direction or [1$\bar{1}$00] ($y$) direction. After adding the spin-orbit coupling $H_{\mathrm{SOC}}$, their two-fold degeneracy is still protected at Γ point. We project onto the same sub-Hilbert space with similar canonical transformation using Eq. S116, where $H^H$ is spanned by the two basis listed above (ordered as given).

After performing the canonical transformation, we obtain the effective Hamiltonian for the AFM MnTe without SOC included at Γ point, derived analytically in the following form:

$$H^\Gamma_{\text{non-SOC}} = \left[c_1\left(k_x^2+k_y^2\right)+c_2k_z^2\right]s_0 \tag{S126}$$

Here, $\boldsymbol{s}$ denotes the spin quantized along the $z$-axis. The independent parameters $c_1$ and $c_2$ are determined through a complex relationship with the tight-binding parameters in Eq. S51 and are distinct from those defined at $A$ point. All terms satisfy the symmetry constraints and are consistent with the $k_z=0$ limit presented in the author's earlier work [6].

Once we add the on-site SOC matrix given by Eq. IV, there appears the correction terms which we derived up to linear order of SOC, in both cases with Néel vector along [11$\bar{2}$0] ($x$) direction, or [1$\bar{1}$00] ($y$) direction.

$$H^\Gamma_{[11\bar{2}0]} = H^\Gamma_{\text{non-SOC}}+\gamma_1k_xk_ys_z \tag{S127}$$

$$H^\Gamma_{[1\bar{1}00]} = H^\Gamma_{\text{non-SOC}}+\frac{\gamma_1}{2}\left(k_x^2-k_y^2\right)s_z \tag{S128}$$

Here, $\gamma_1$ is a parameter which depends on the parameters in Eq. S51 in complicated form. Importantly, the tight binding calculation shows that $\gamma_1$ term is a first-order correction in SOC, thus this first order term is the dominant contribution for spin-splitting at Γ point. $\gamma_1$ is analytically related between the two cases, as shown in Eqs. S127 and S128.

## VIII. FITTING BAND RESULTS FOR THE EFFECTIVE HAMILTONIAN

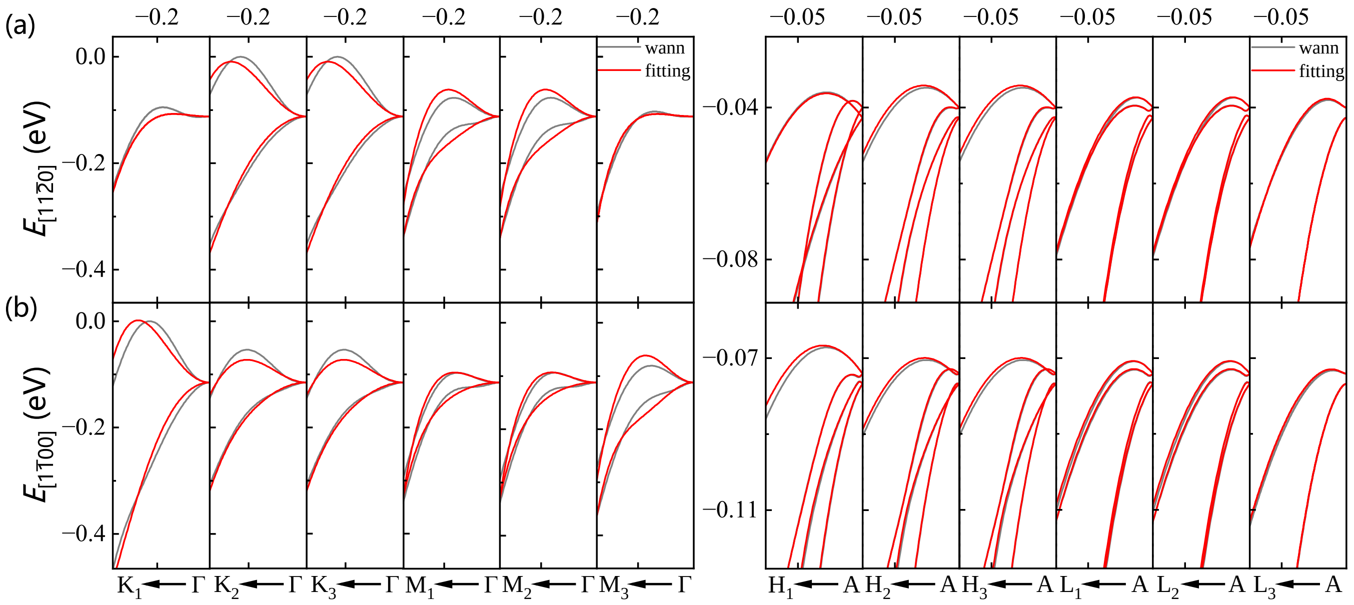


Figure S4. Band structures obtained by fitting using effective Hamiltonian. Red lines indicate the fitted curves, while gray lines show the DFT results. (a) Néel vector aligned along the $[11\bar{2}0]$ ($x$) direction. (b) Néel vector aligned along the $[1\bar{1}00]$ ($y$) direction. The left and right panels show the regions near the Γ and A points, respectively.


[1] J. C. Slater and G. F. Koster, Simplified LCAO Method for the Periodic Potential Problem, Physical Review **94**, 1498 (1954).

[2] S. Konschuh, M. Gmitra, and J. Fabian, Tight-binding theory of the spin-orbit coupling in graphene, Phys. Rev. B **82**, 245412 (2010).

[3] D. Kriegner, K. Výborný, K. Olejník, H. Reichlová, V. Novák, X. Marti, J. Gazquez, V. Saidl, P. Němec, V. V. Volobuev, G. Springholz, V. Holý, and T. Jungwirth, Multiple-stable anisotropic magnetoresistance memory in antiferromagnetic MnTe, Nature Communications **7**, 11623 (2016).

[4] J. R. Schrieffer and P. A. Wolff, Relation between the Anderson and Kondo Hamiltonians, Phys. Rev. **149**, 491 (1966).

[5] C.-C. Liu, H. Jiang, and Y. Yao, Low-energy effective Hamiltonian involving spin-orbit coupling in silicene and two-dimensional germanium and tin, Phys. Rev. B **84**, 195430 (2011).

[6] G. Yin, J.-X. Yu, Y. Liu, R. K. Lake, J. Zang, and K. L. Wang, Planar Hall Effect in Antiferromagnetic MnTe Thin Films, Physical Review Letters **122**, 106602 (2019).
